# Supplementary material for: Continual Source-Free Unsupervised Domain Adaptation
Source: arXiv:2304.07374 source file (2023-04-14)
Supplement: Supplementary file 1 [file figure_supp_neg.tex]

%%%%%%%%%%%%%%%%%%%%%%%%%%%%%%%%%%%%%%%%%%%%%%%%%%%%%%%%%%%%%%%%%%%
\begin{figure*}[!t]
%
%\setlength{\abovecaptionskip}{3pt}
% \setlength{\belowcaptionskip}{-5pt}
% \captionsetup{font=small}
\centering
%%%%%%%%%%%%%%%%%%%%%%%%%%%%%%%
\hspace{0.2em}
\begin{subfigure}{0.3\textwidth}
\centering
\captionsetup{font=small}
\includegraphics[width=0.8\linewidth]{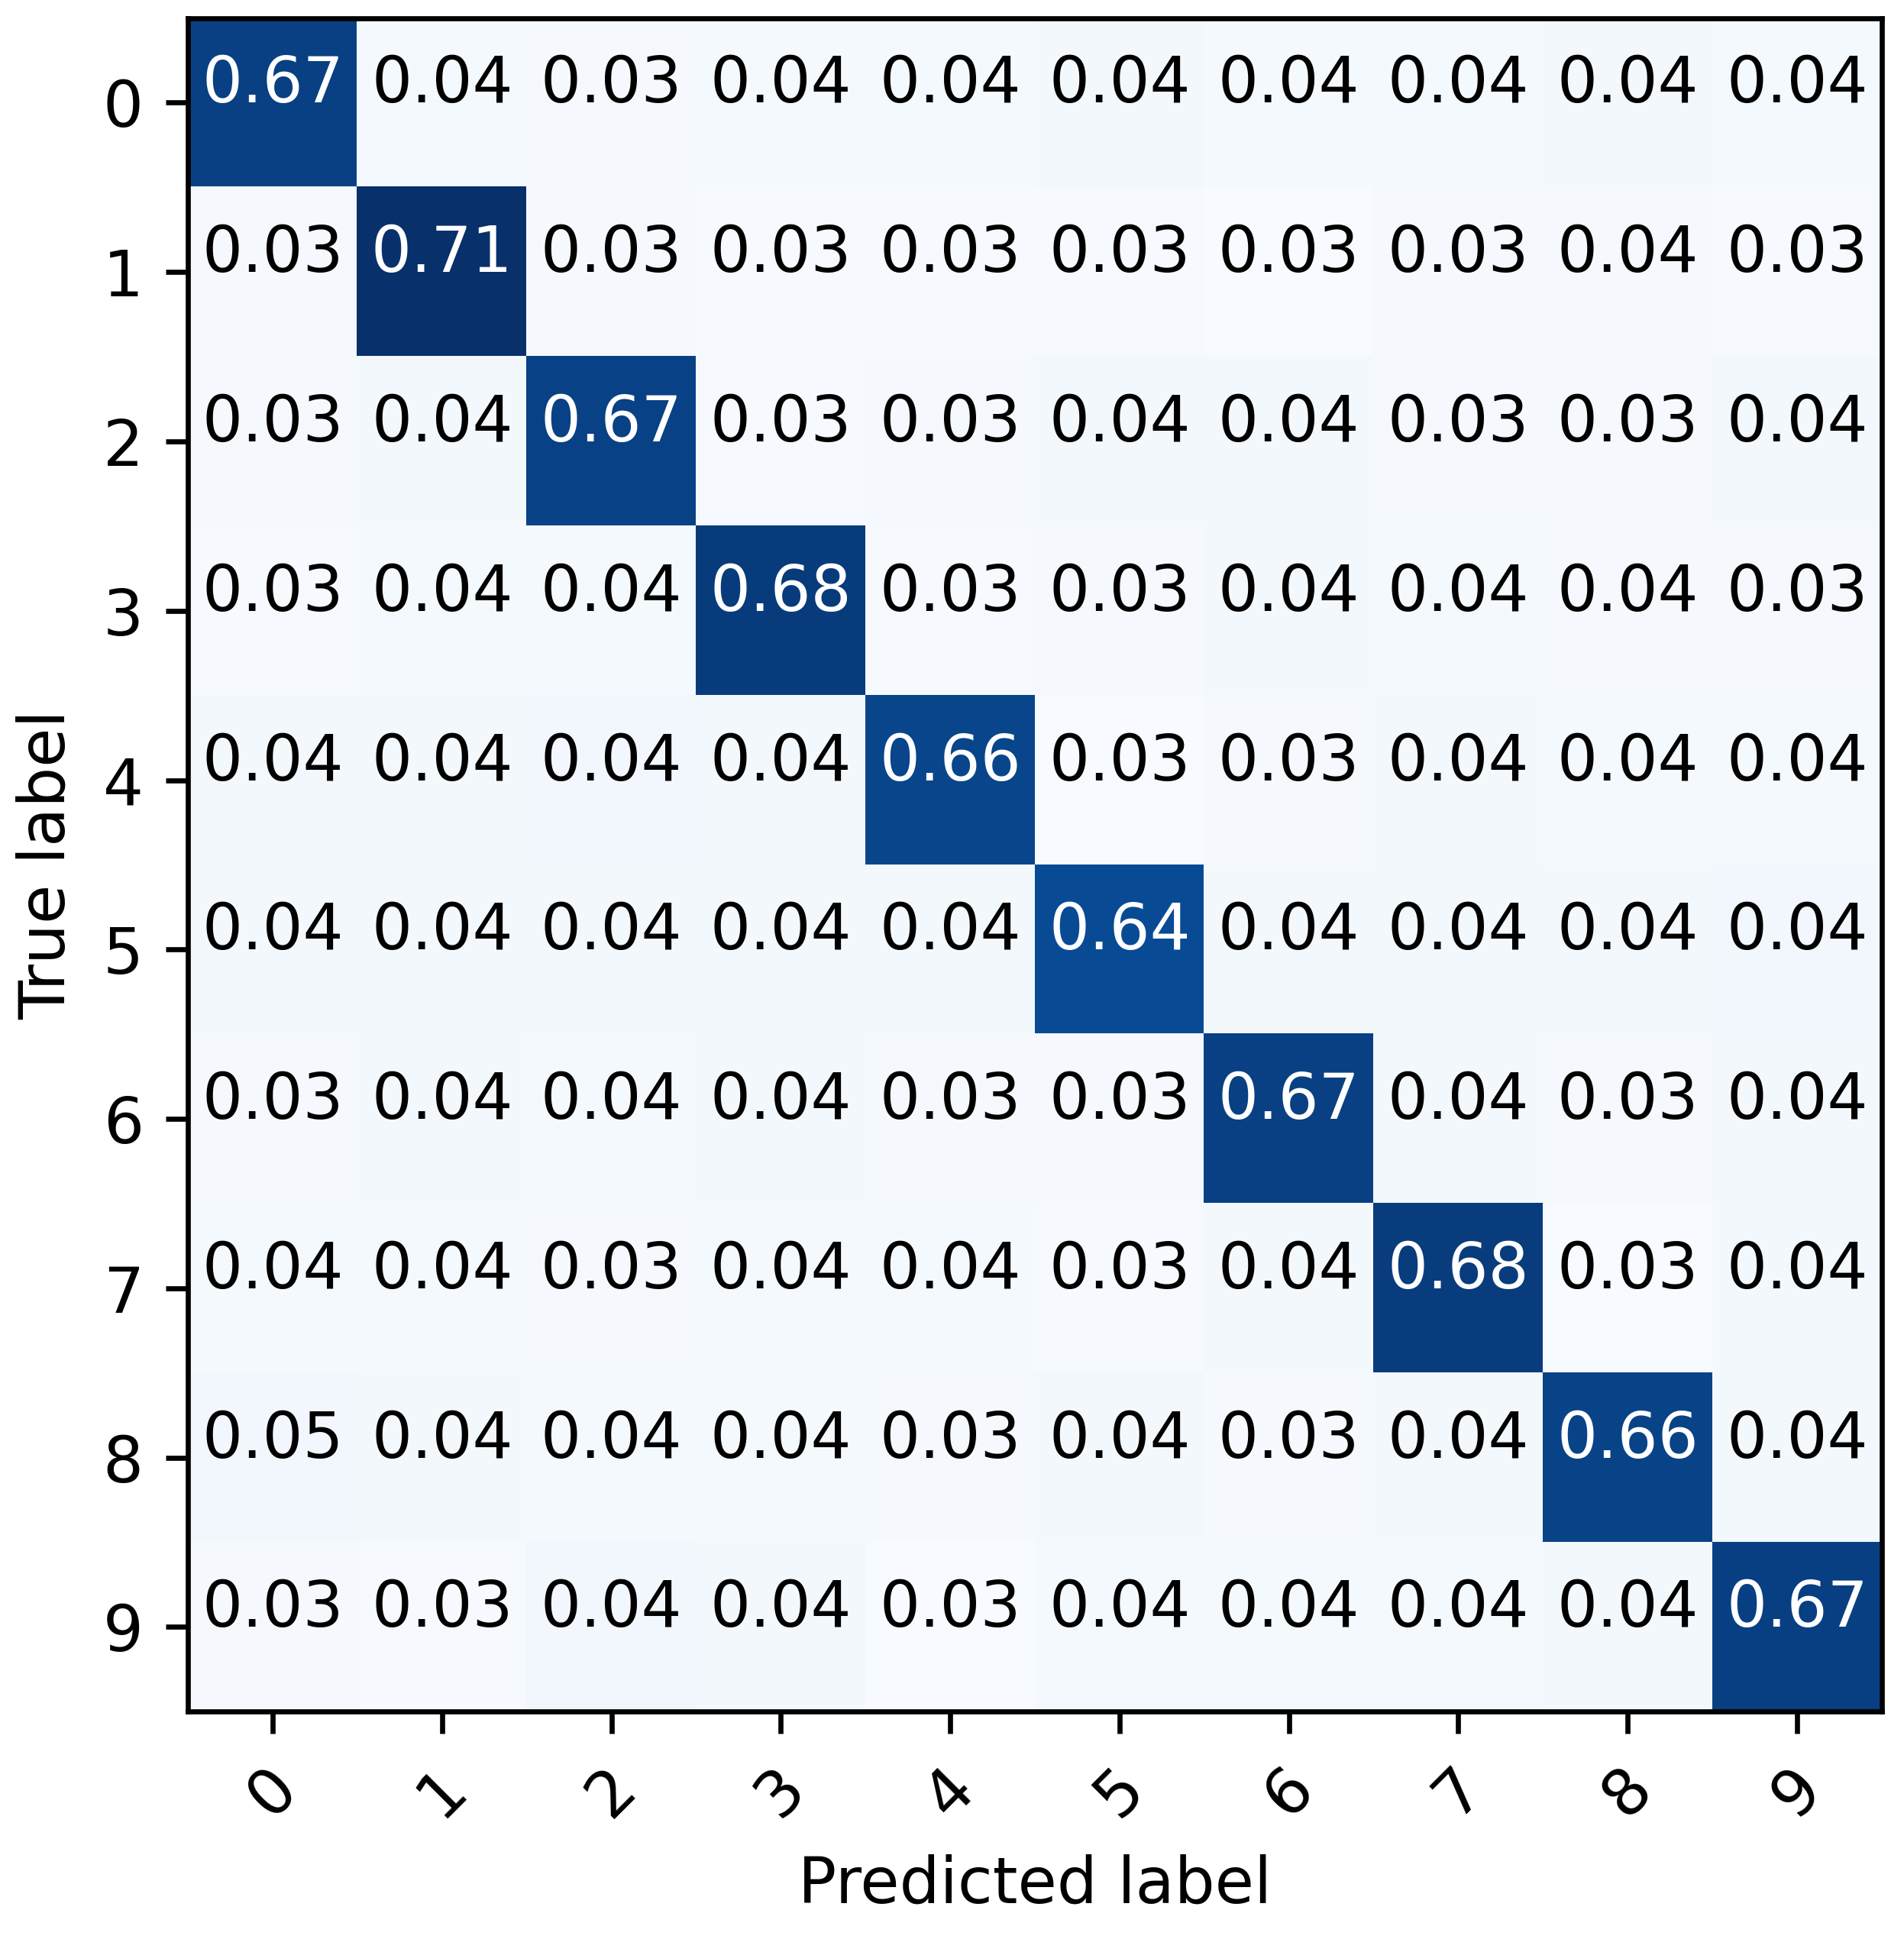}
\end{subfigure}
\hspace{0.6em}
\begin{subfigure}{0.3\textwidth}
\centering
\captionsetup{font=small}
\includegraphics[width=0.8\linewidth]{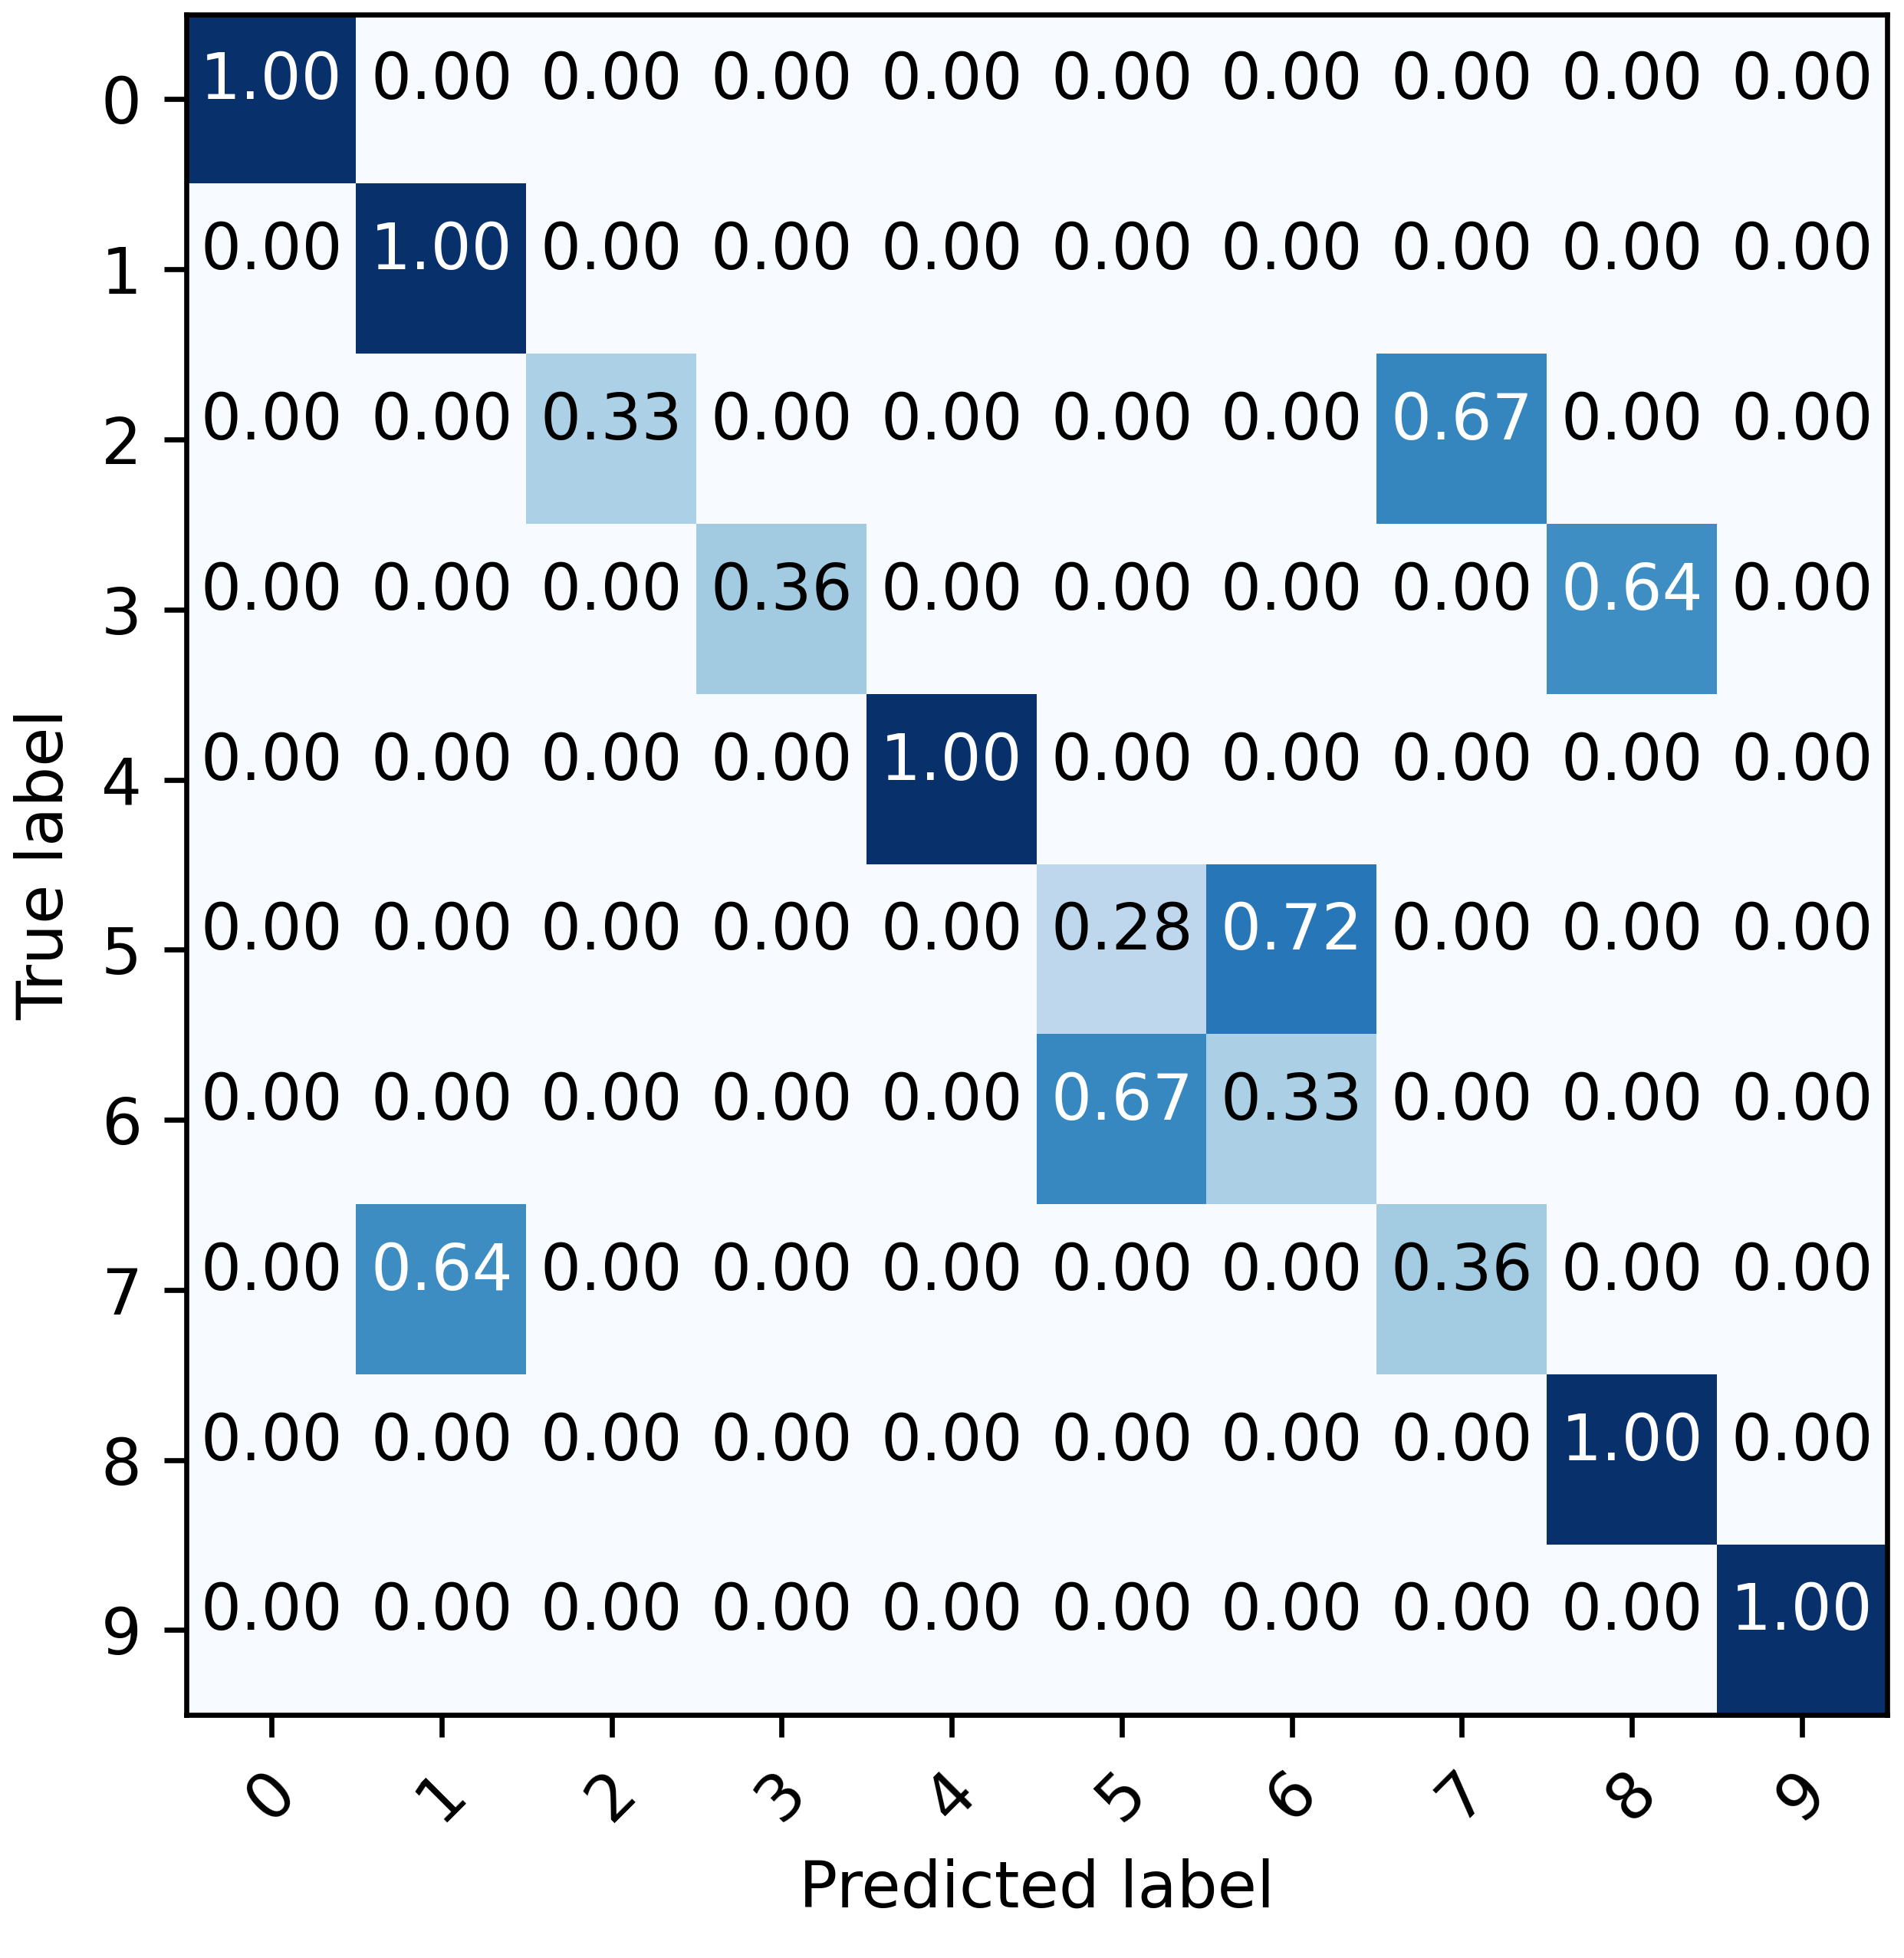}
\end{subfigure}
\hspace{0.6em}
\begin{subfigure}{0.3\textwidth}
\centering
\captionsetup{font=small}
\includegraphics[width=0.8\linewidth]{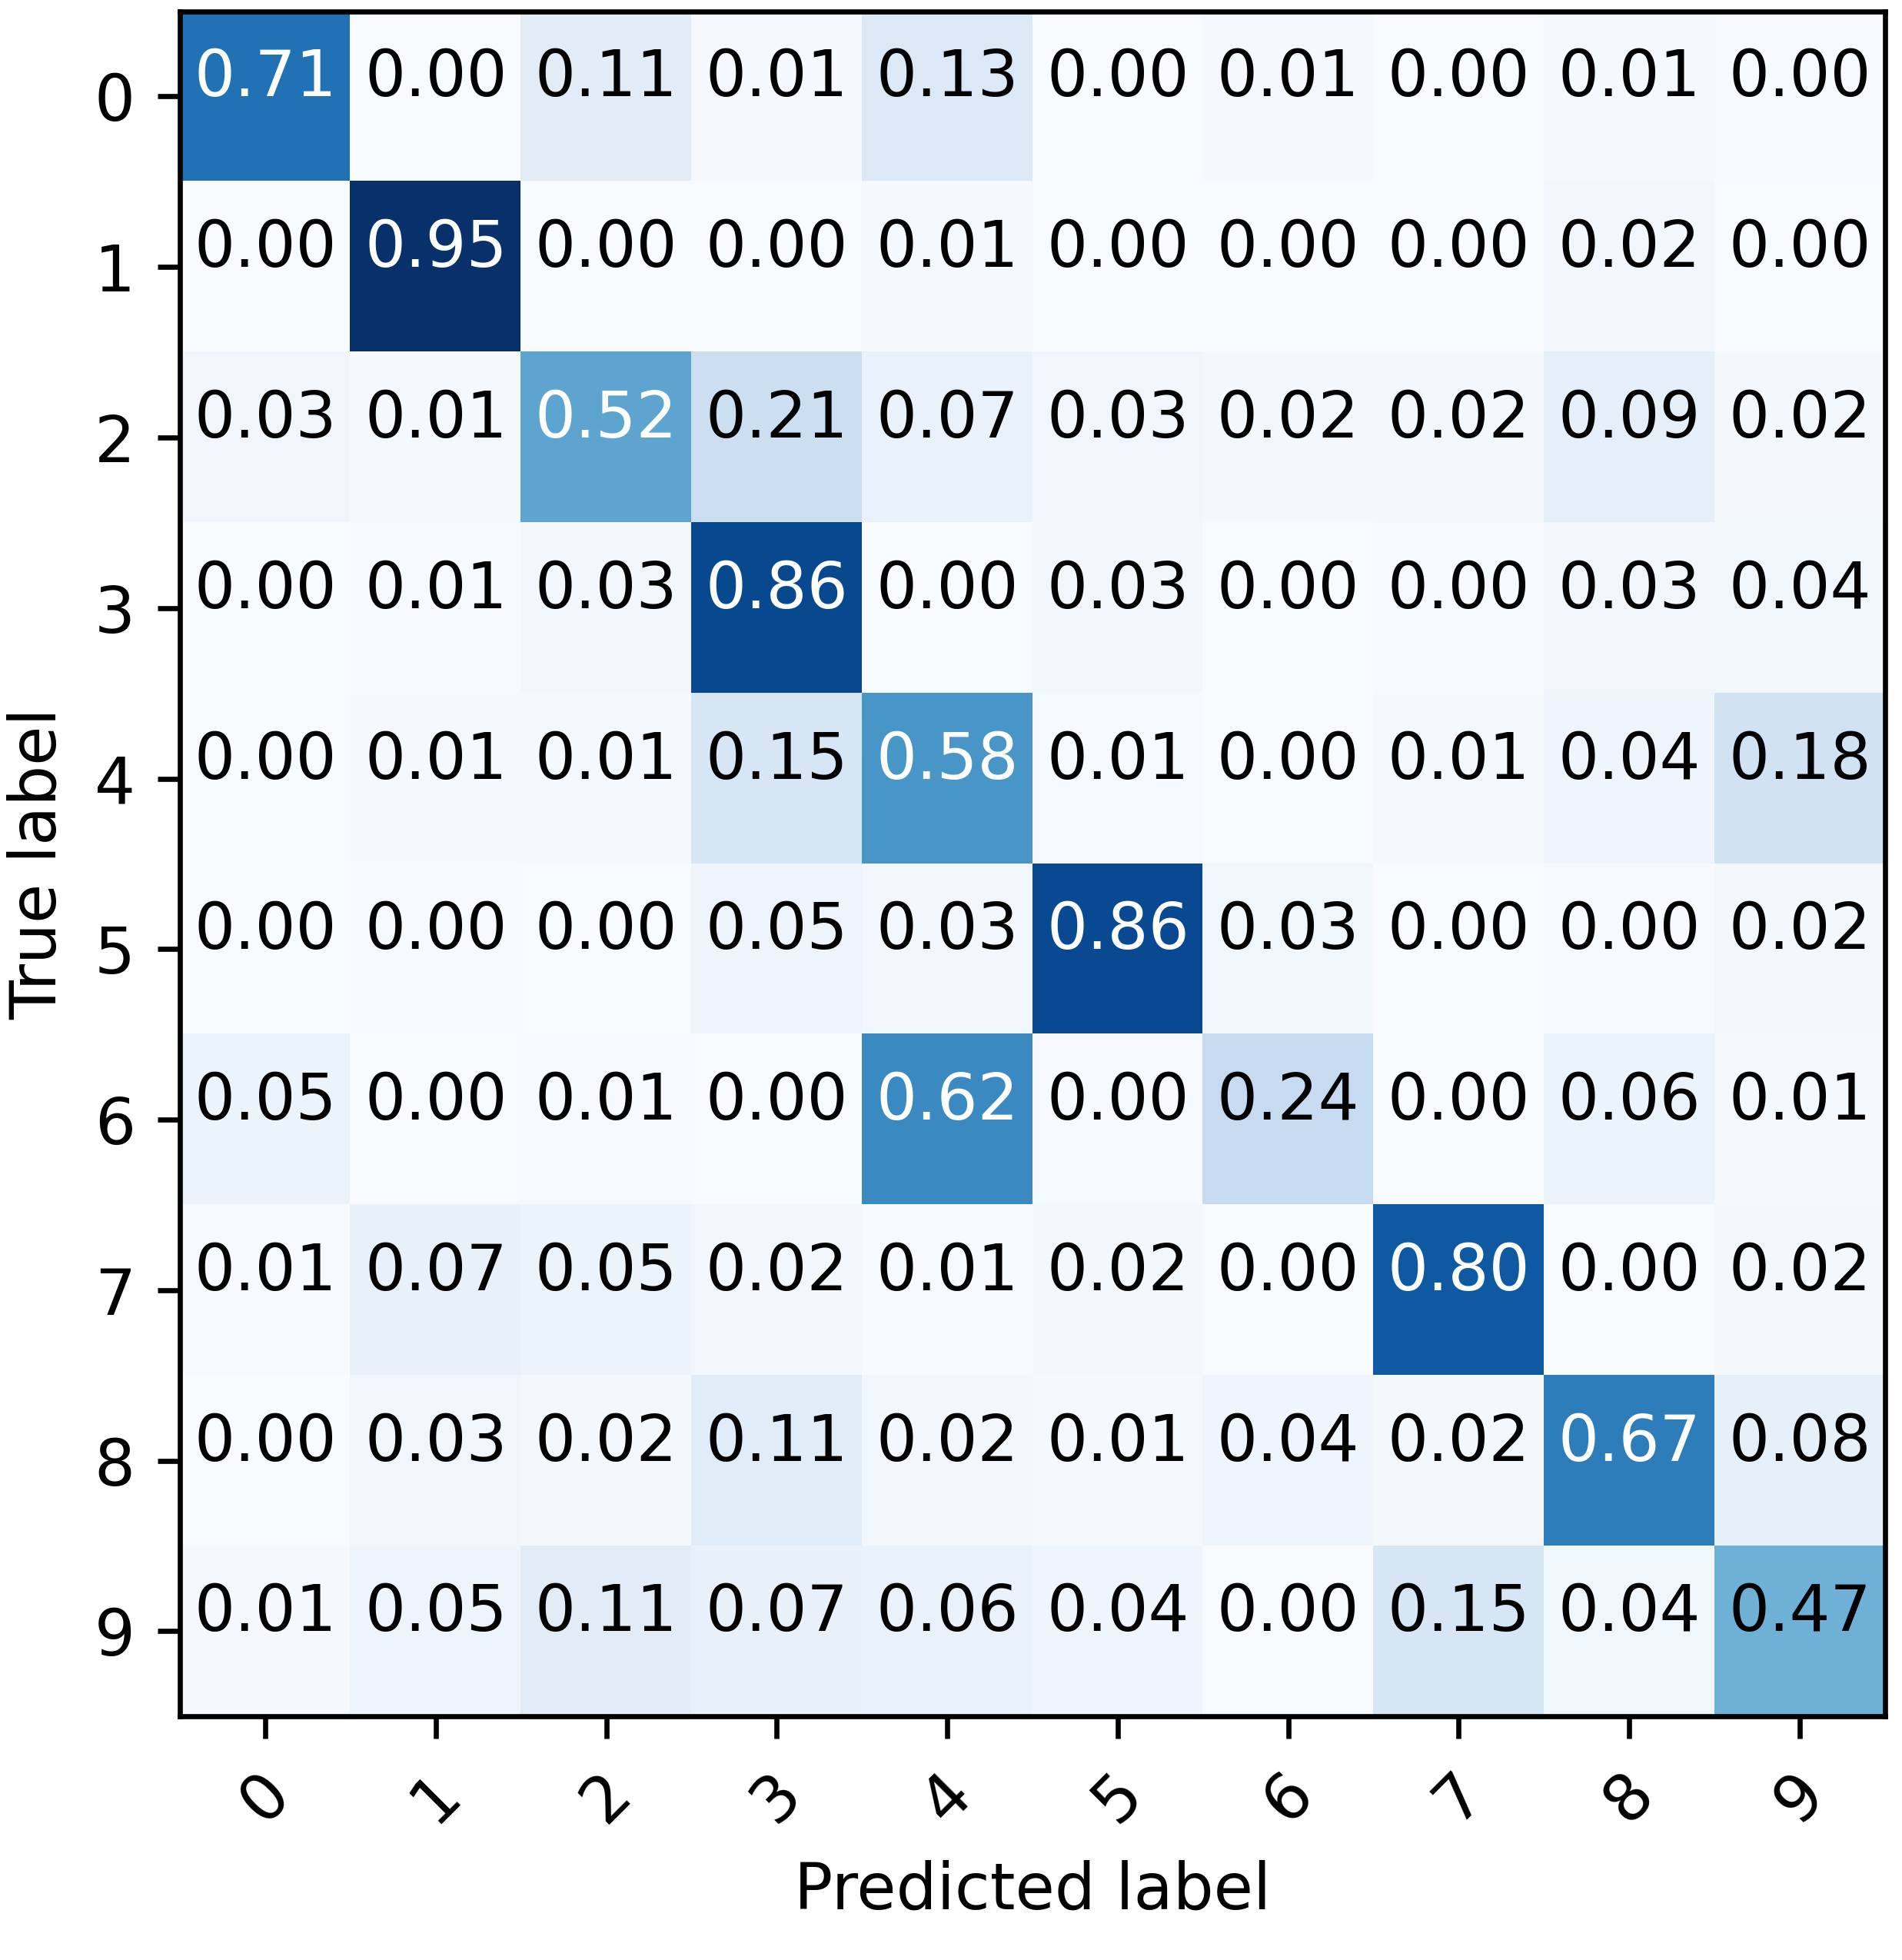}
\end{subfigure}
% \\
% %
% \begin{subfigure}{0.32\textwidth}
% \centering
% \captionsetup{font=small}
% \includegraphics[width=\linewidth]{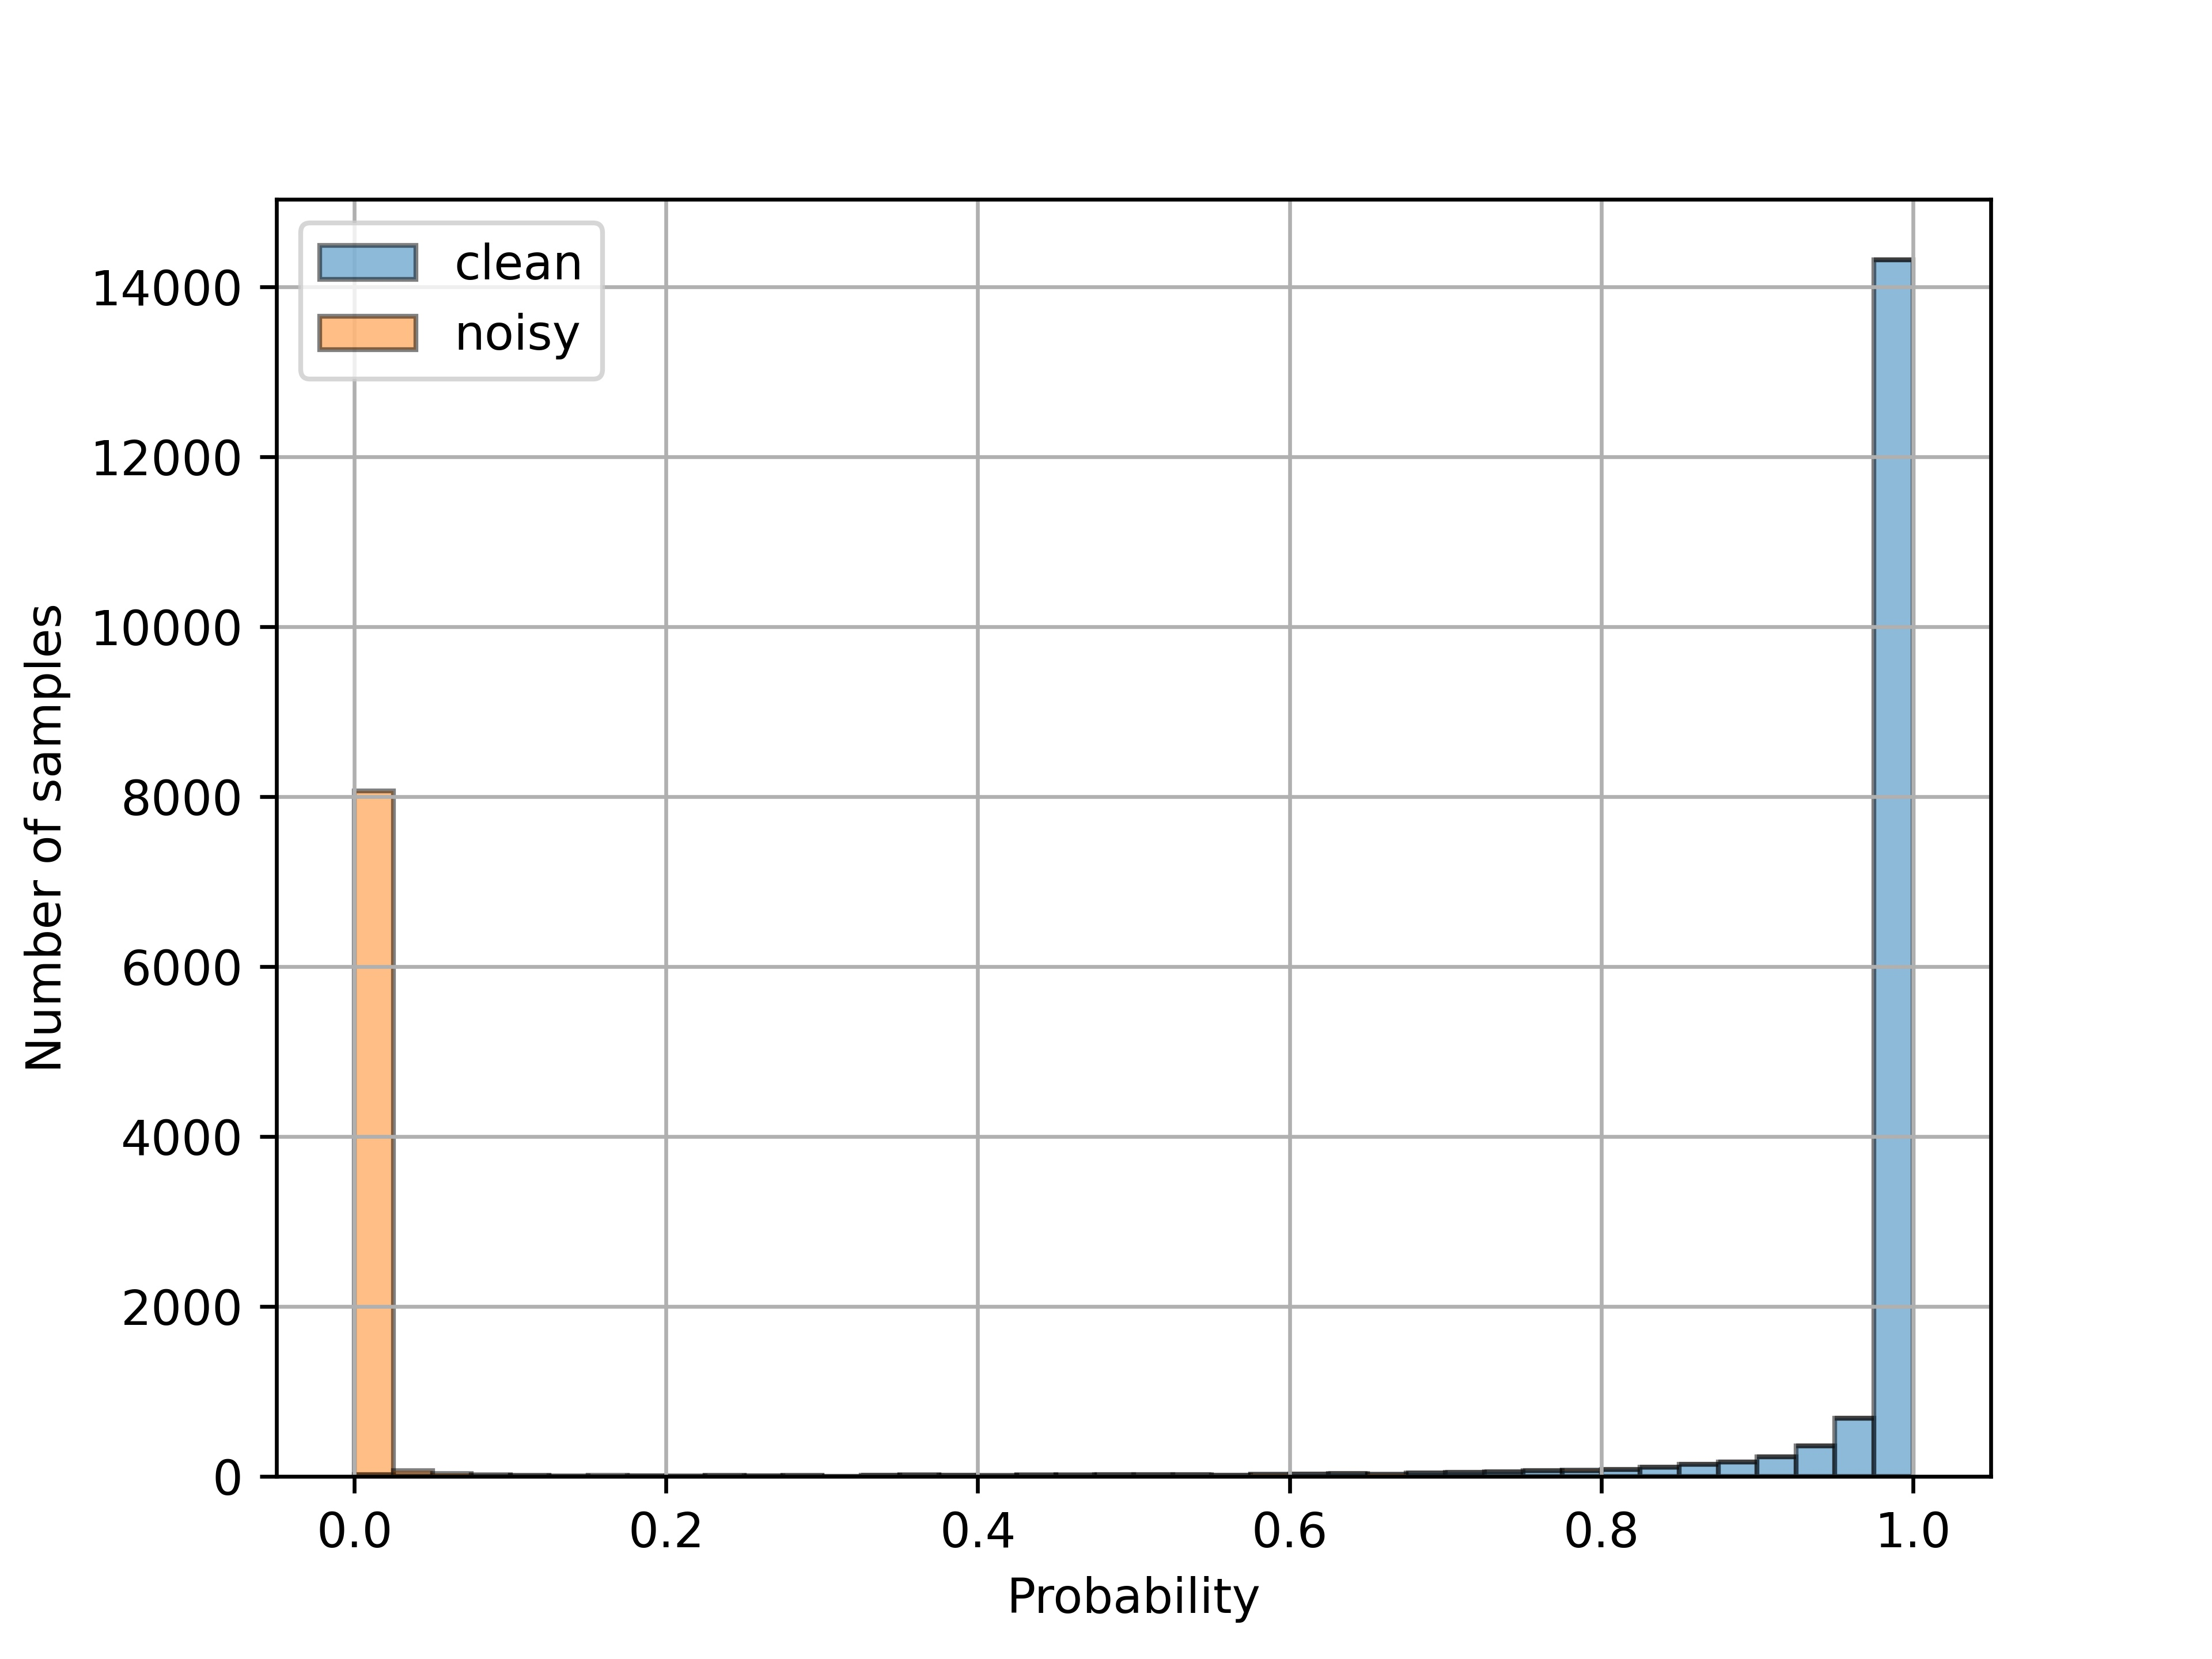}
% \end{subfigure}
% \begin{subfigure}{0.32\textwidth}
% \centering
% \captionsetup{font=small}
% \includegraphics[width=\linewidth]{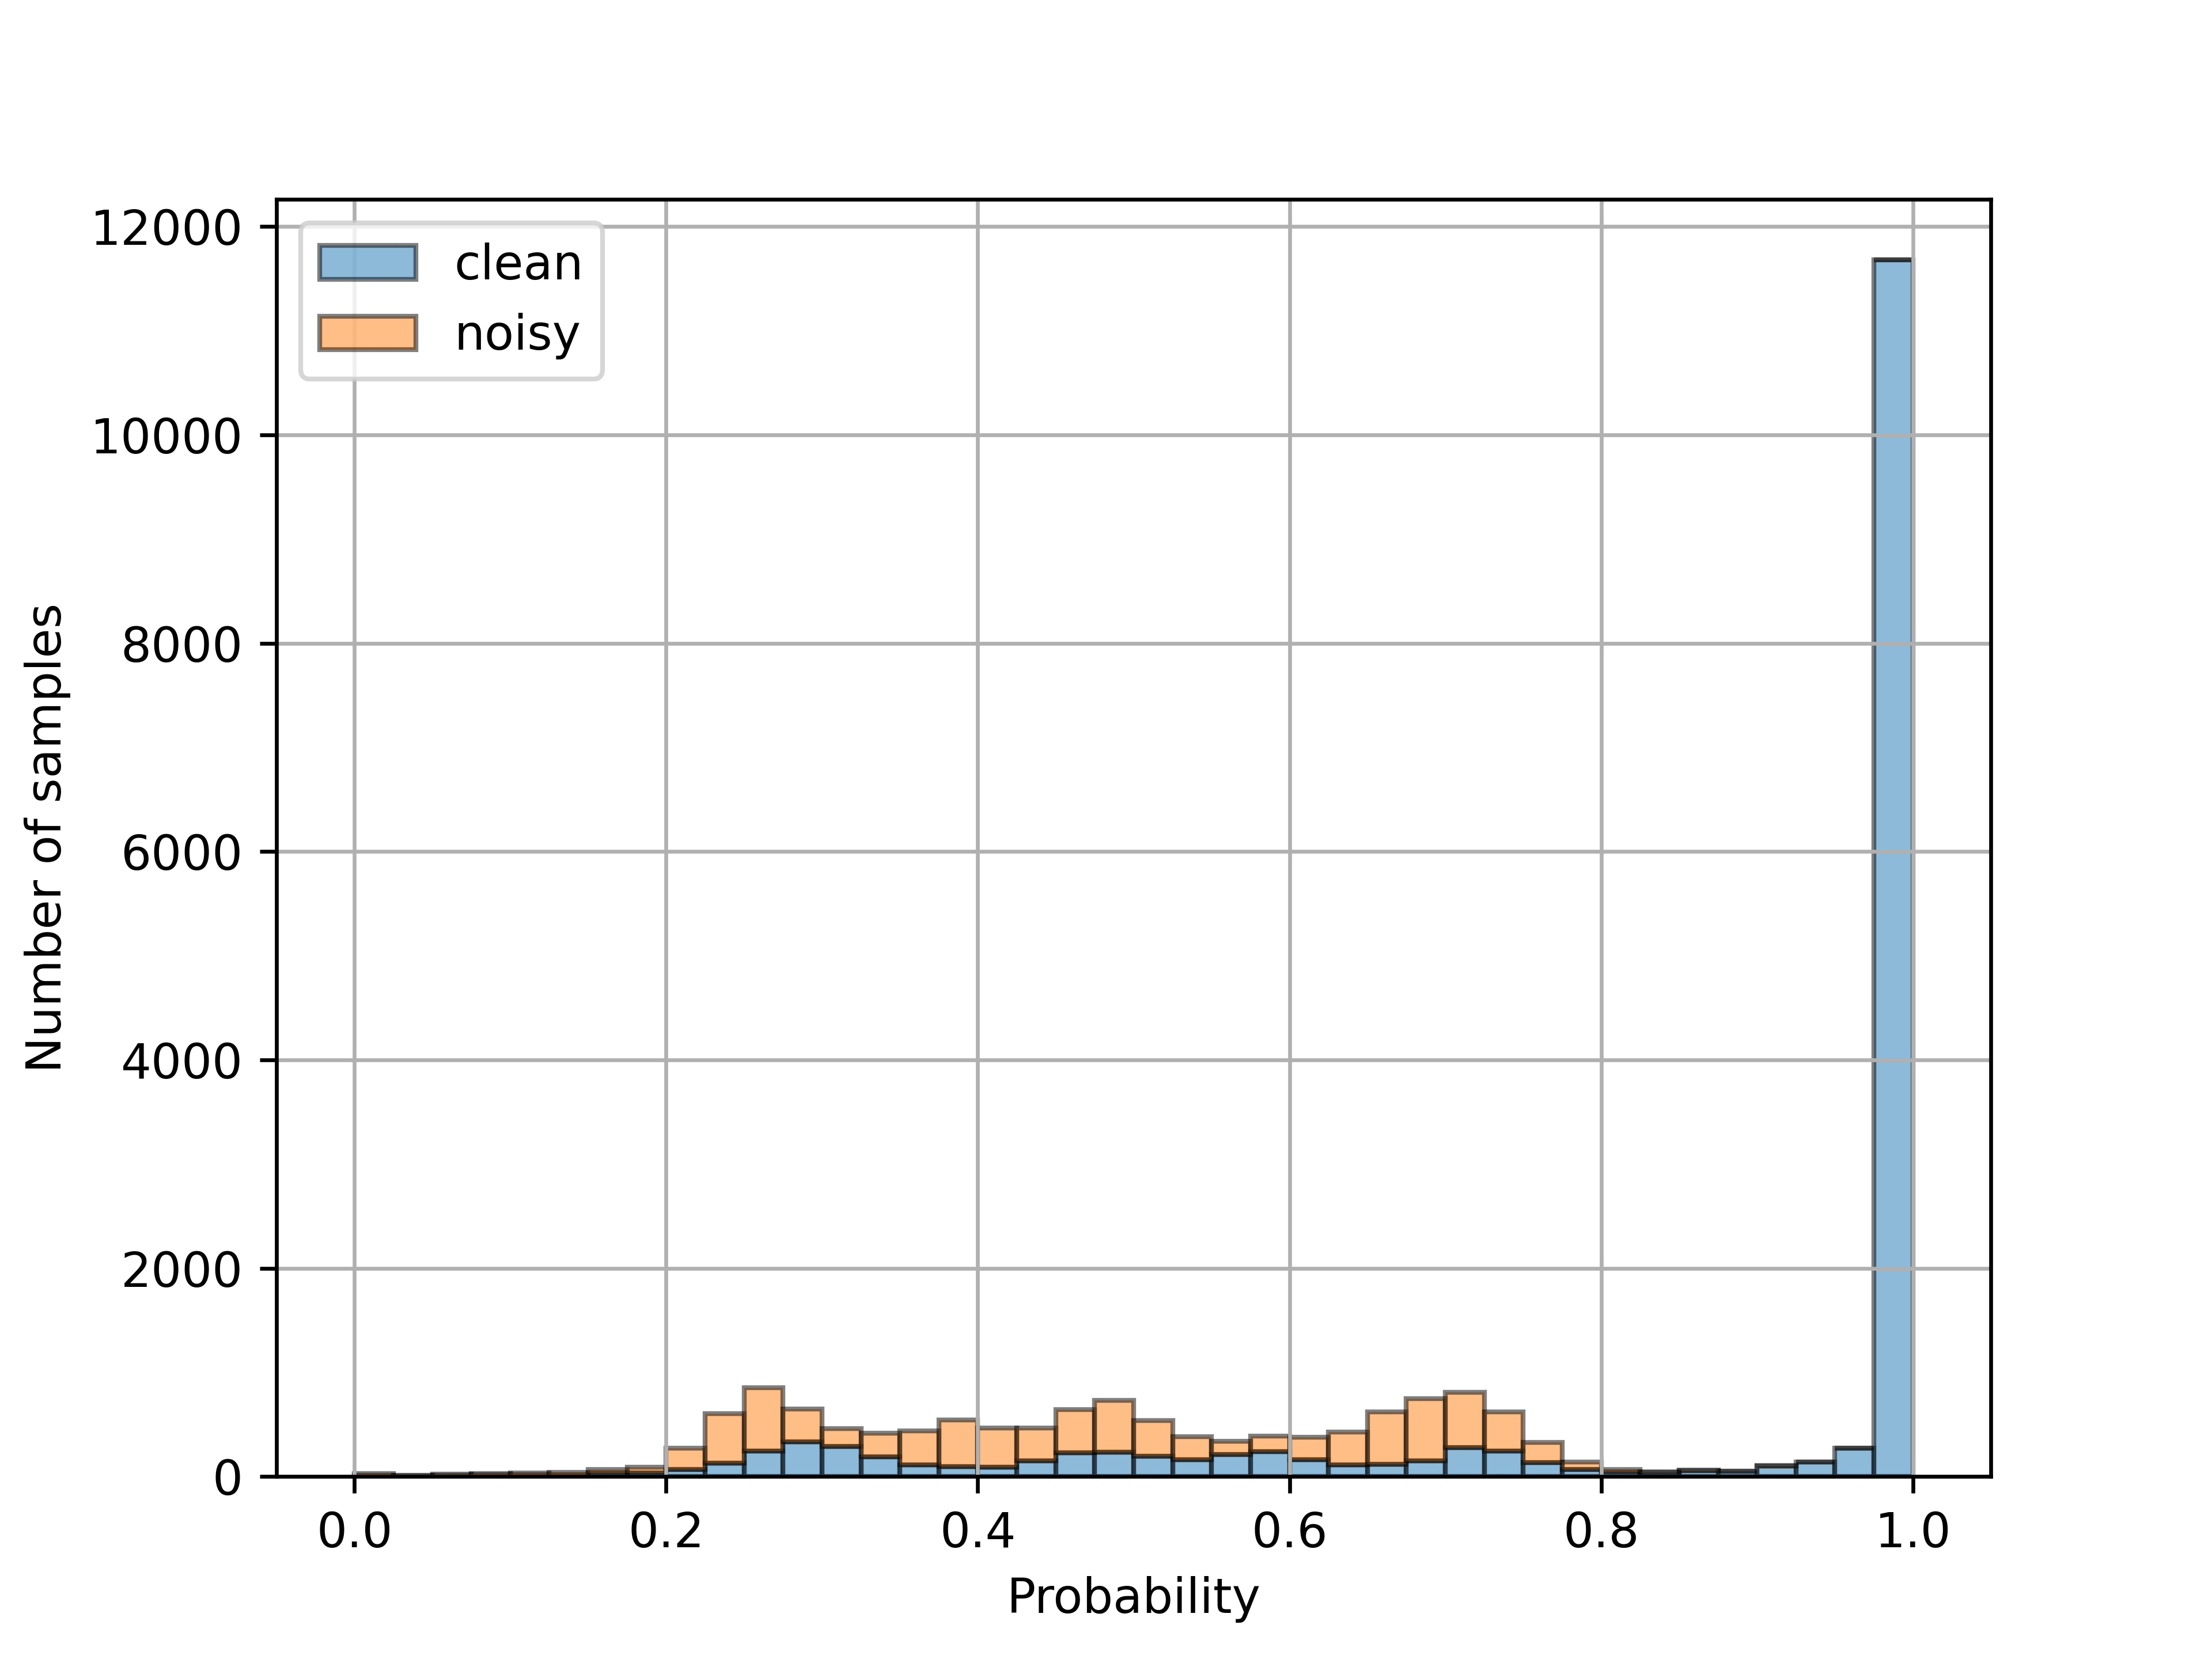}
% \end{subfigure}
% \begin{subfigure}{0.32\textwidth}
% \centering
% \captionsetup{font=small}
% \includegraphics[width=\linewidth]{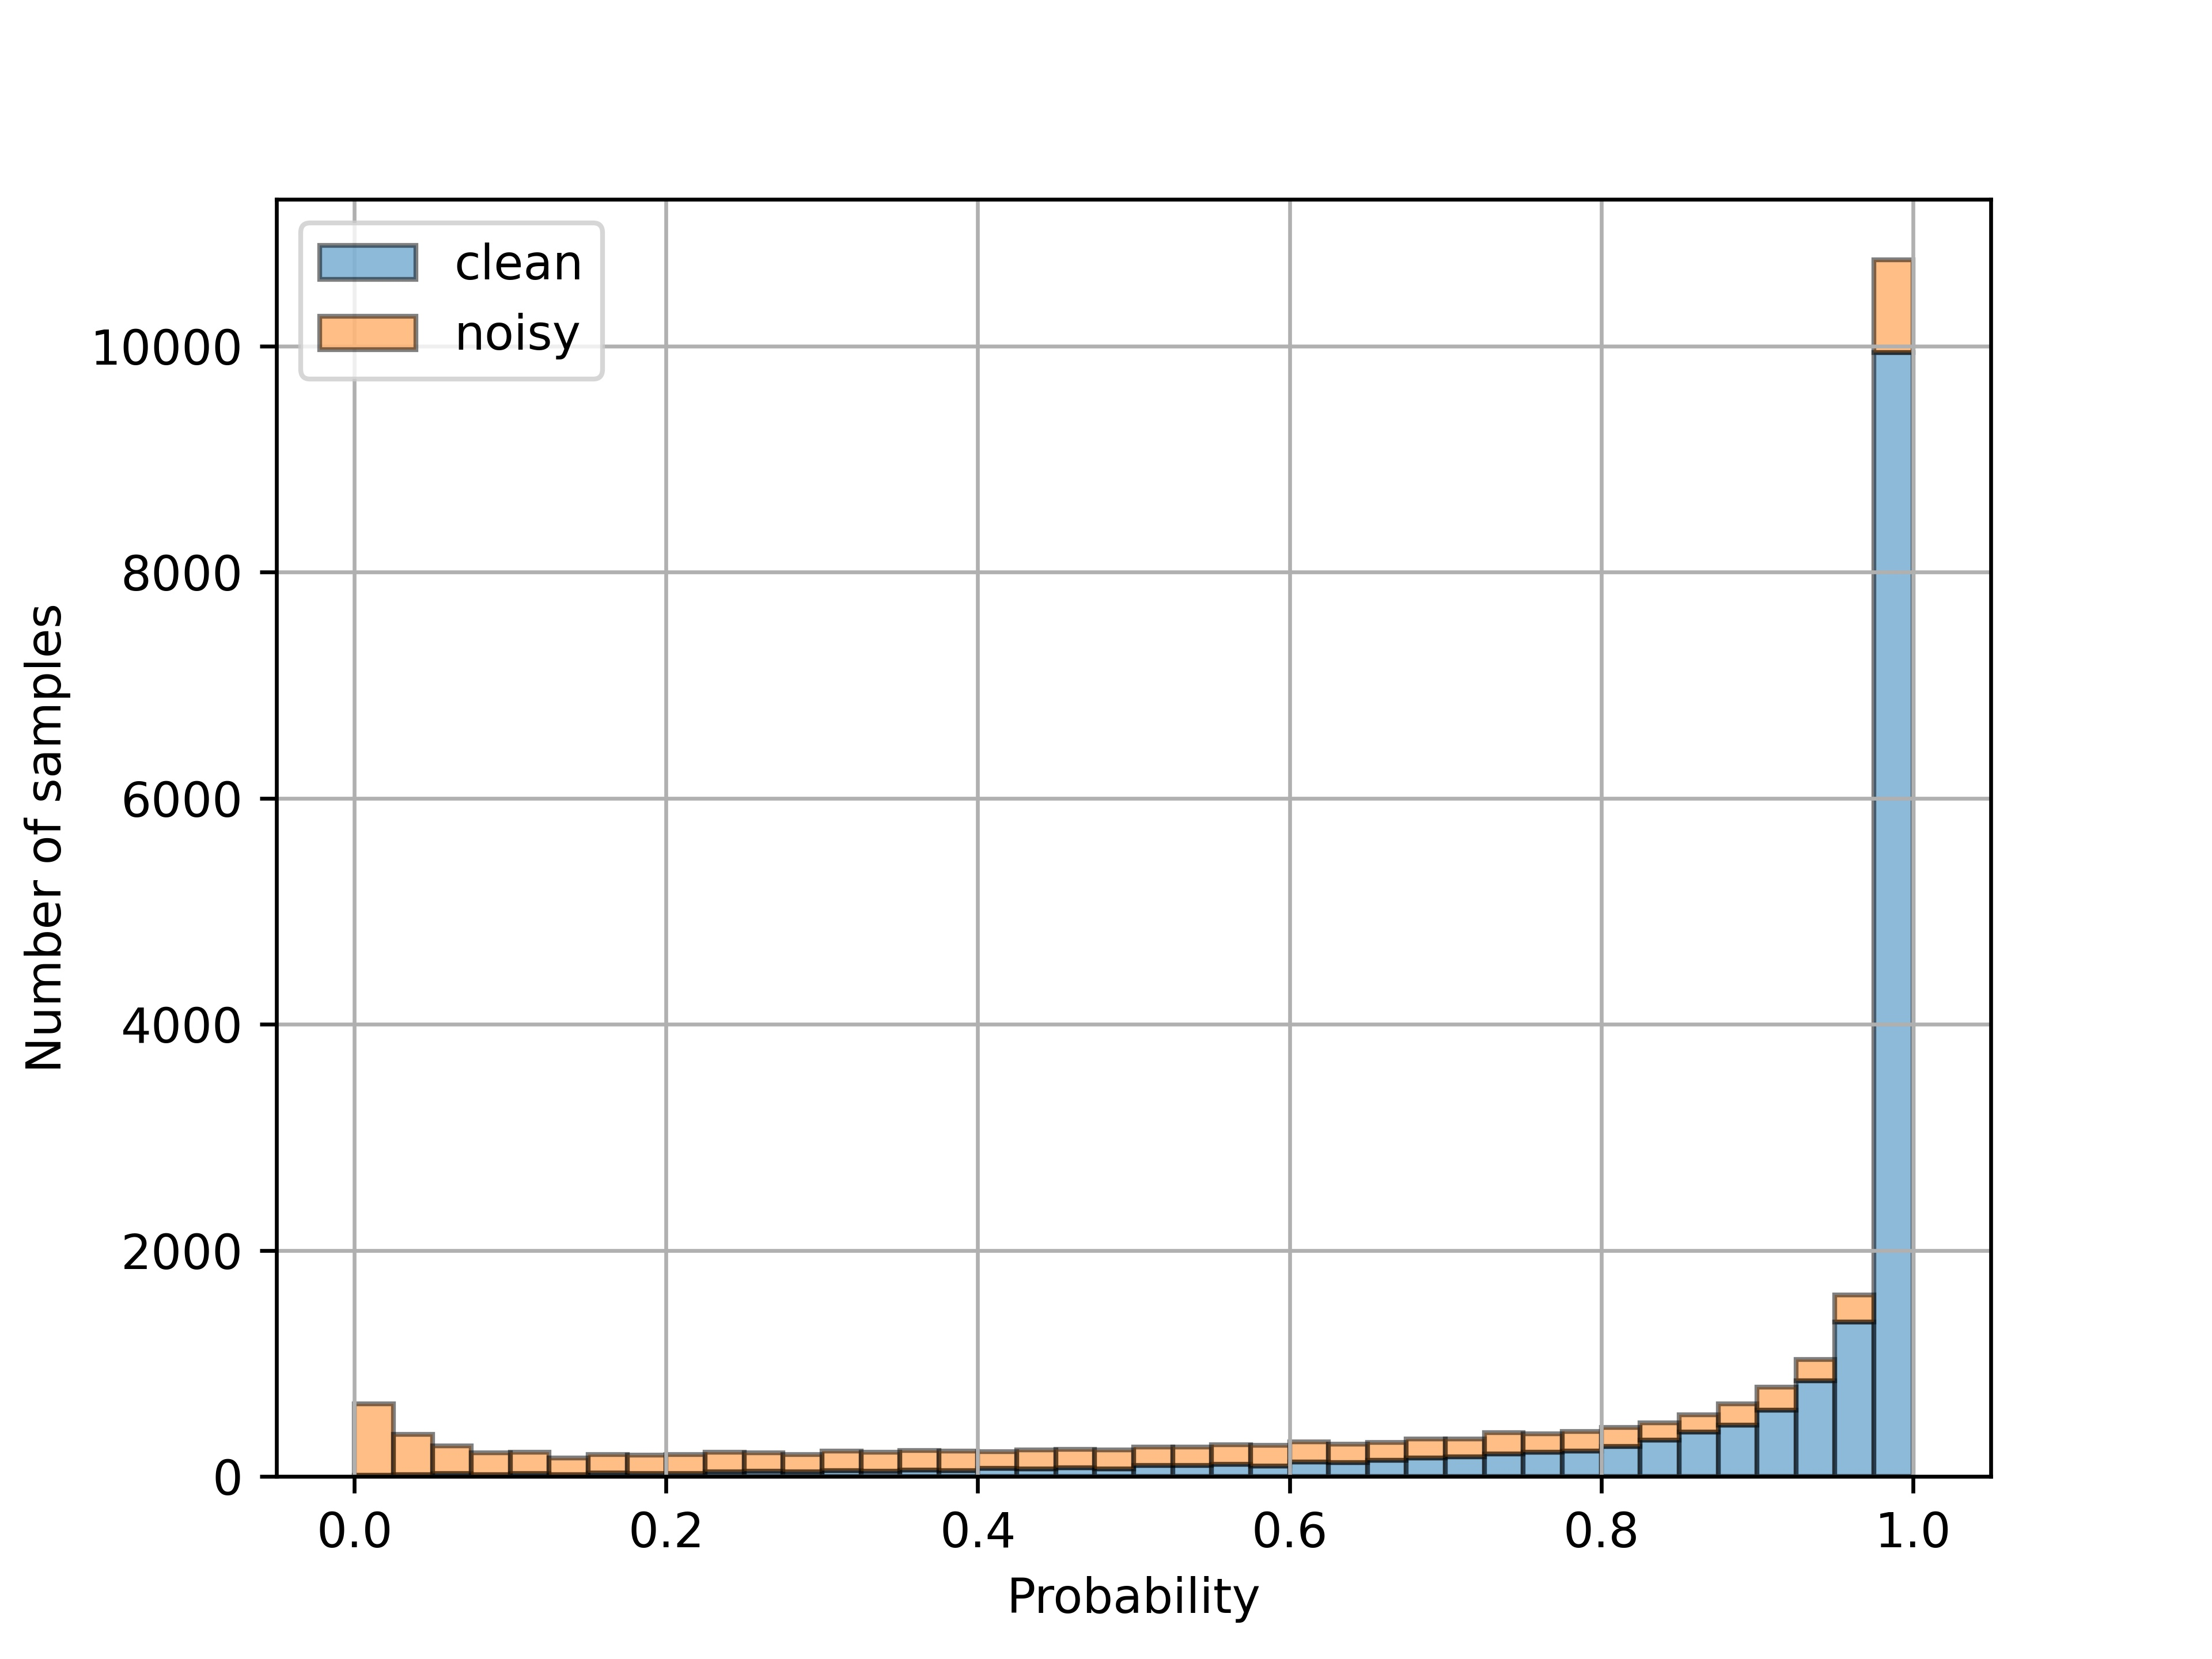}
% \end{subfigure}
\\
\begin{subfigure}{0.31\textwidth}
\centering
\captionsetup{font=small}
\includegraphics[width=\linewidth]{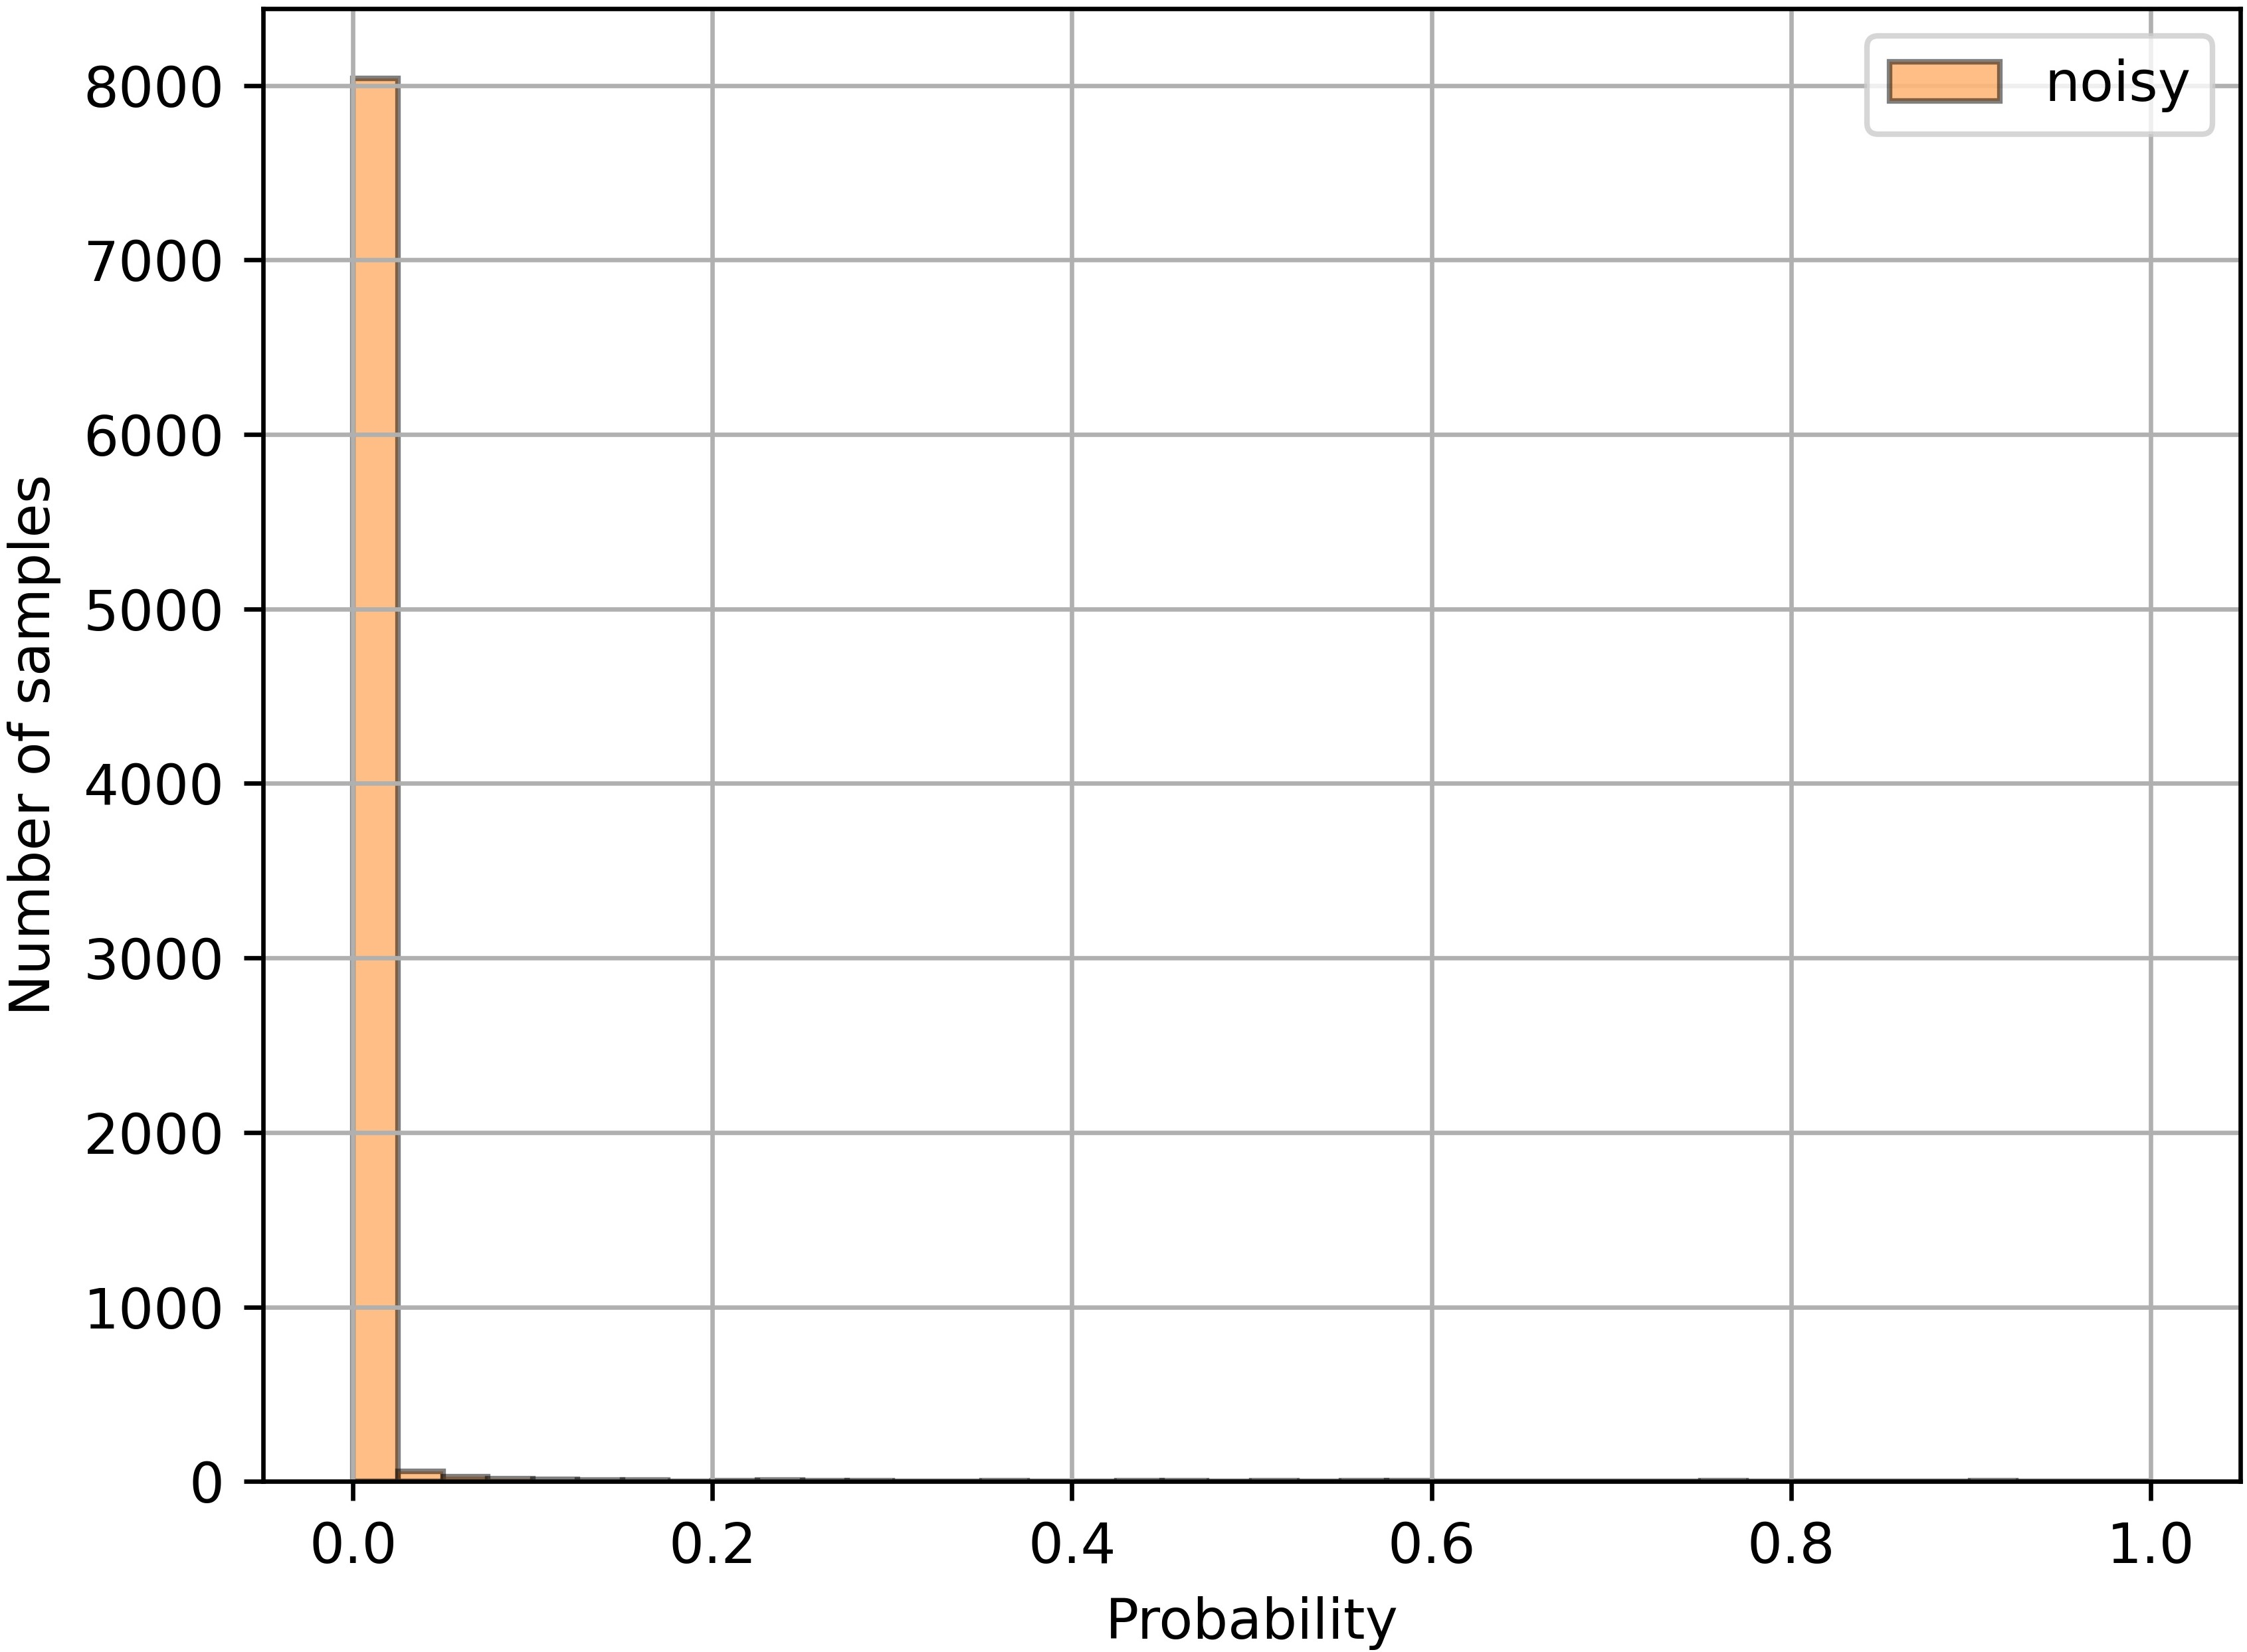}
% \caption{Symmetric-Noise}
% \label{NL:symm}
\end{subfigure}
\hspace{0.3em}
\begin{subfigure}{0.305\textwidth}
\centering
\captionsetup{font=small}
\includegraphics[width=\linewidth]{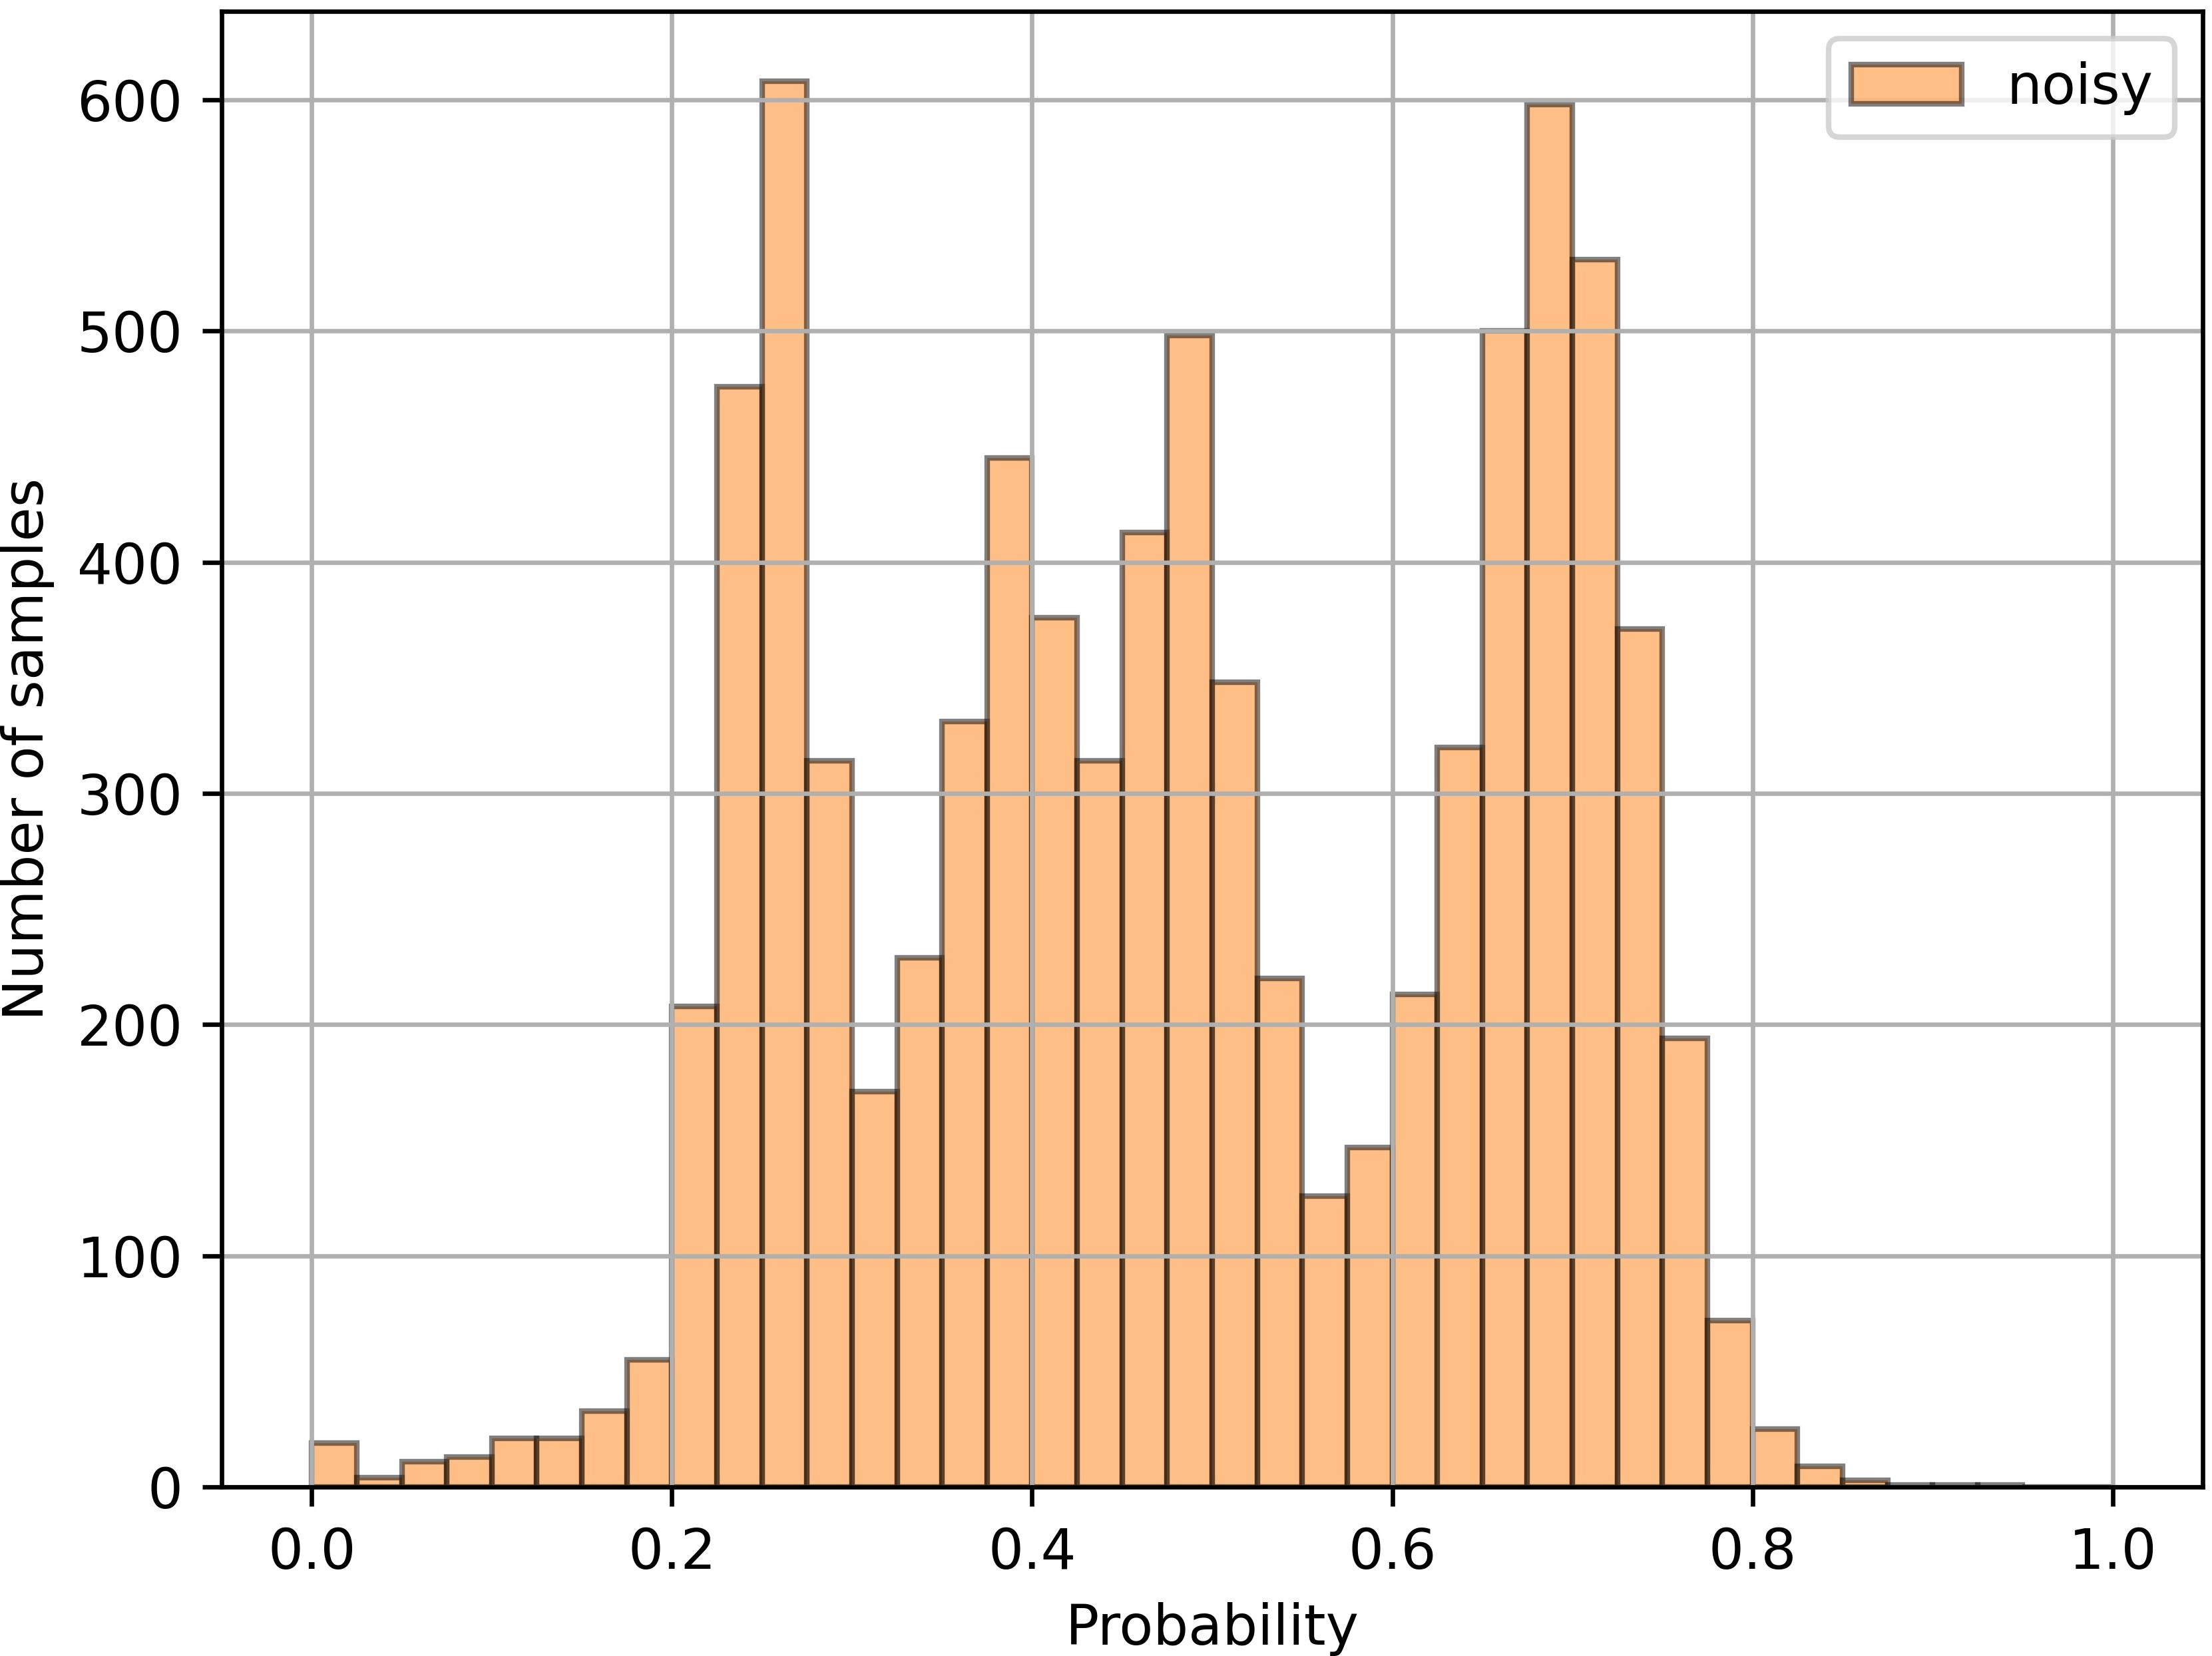}
% \caption{Asymmetric-Noise}
% \label{NL:asymm}
\end{subfigure}
\hspace{0.3em}
\begin{subfigure}{0.305\textwidth}
\centering
\captionsetup{font=small}
\includegraphics[width=\linewidth]{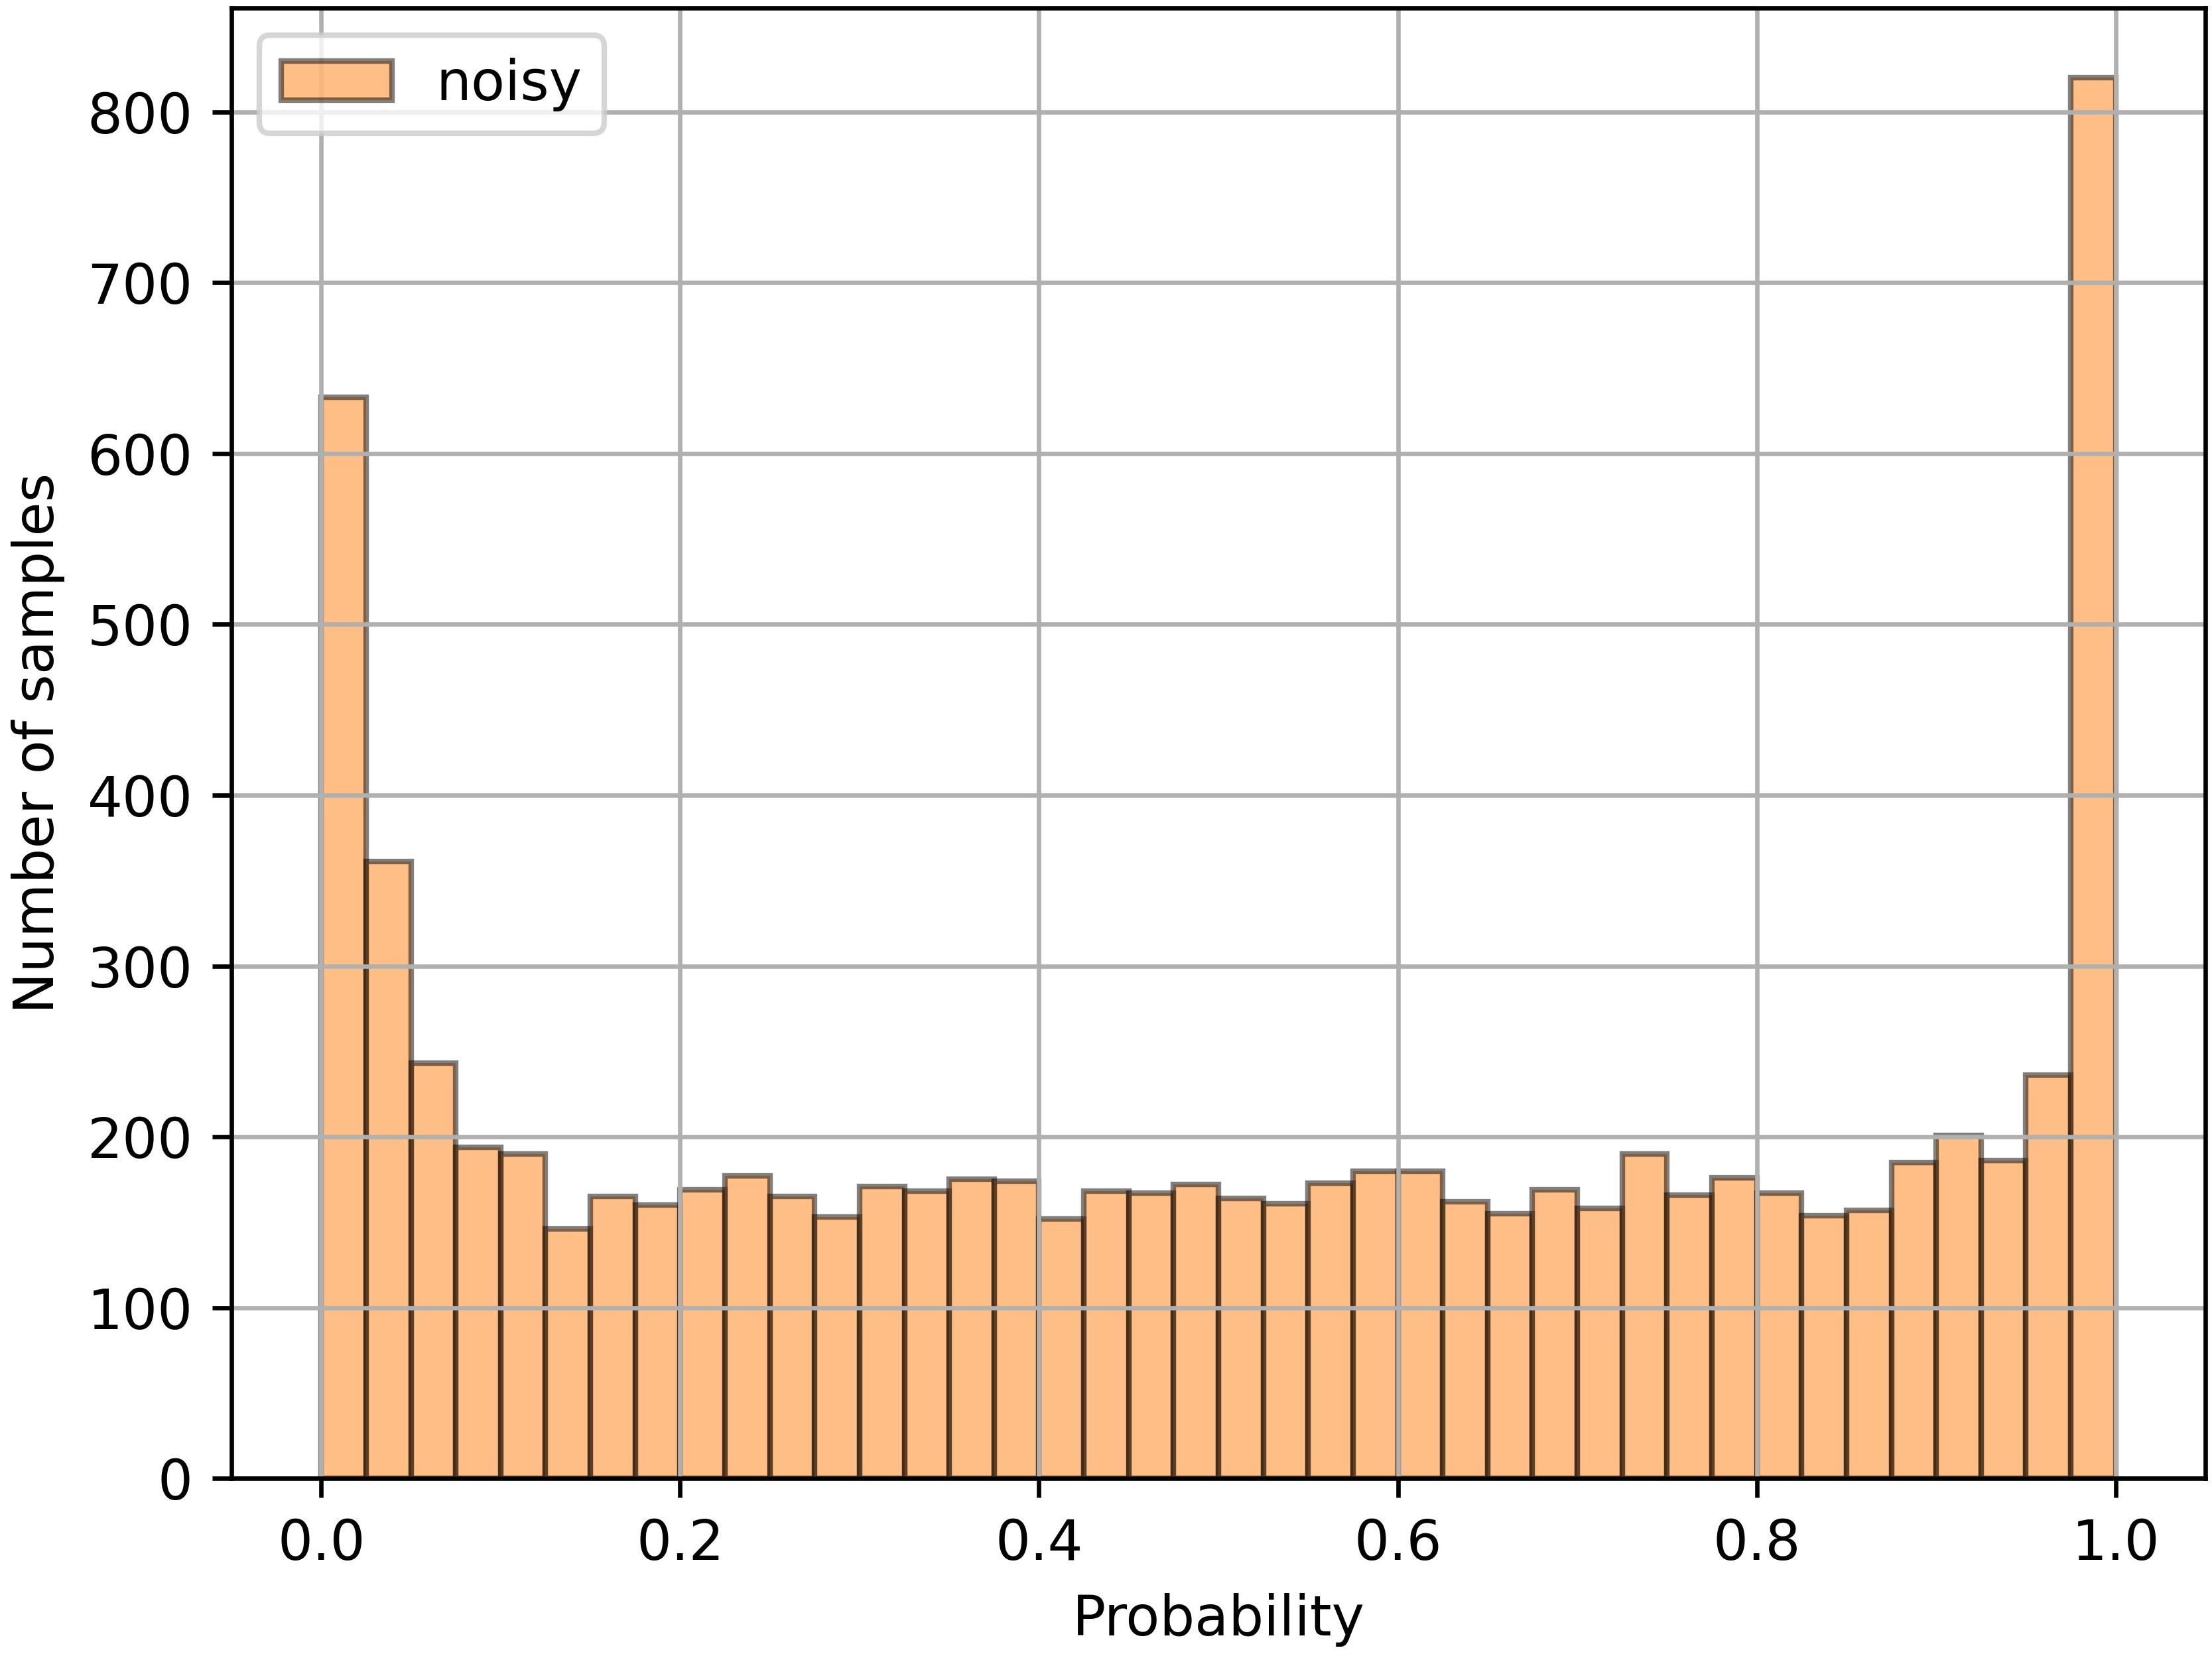}
% \caption{Shift-Noise}
% \label{NL:shift}
\end{subfigure}
\\
\begin{subfigure}{0.315\textwidth}
\centering
\captionsetup{font=small}
\includegraphics[width=\linewidth]{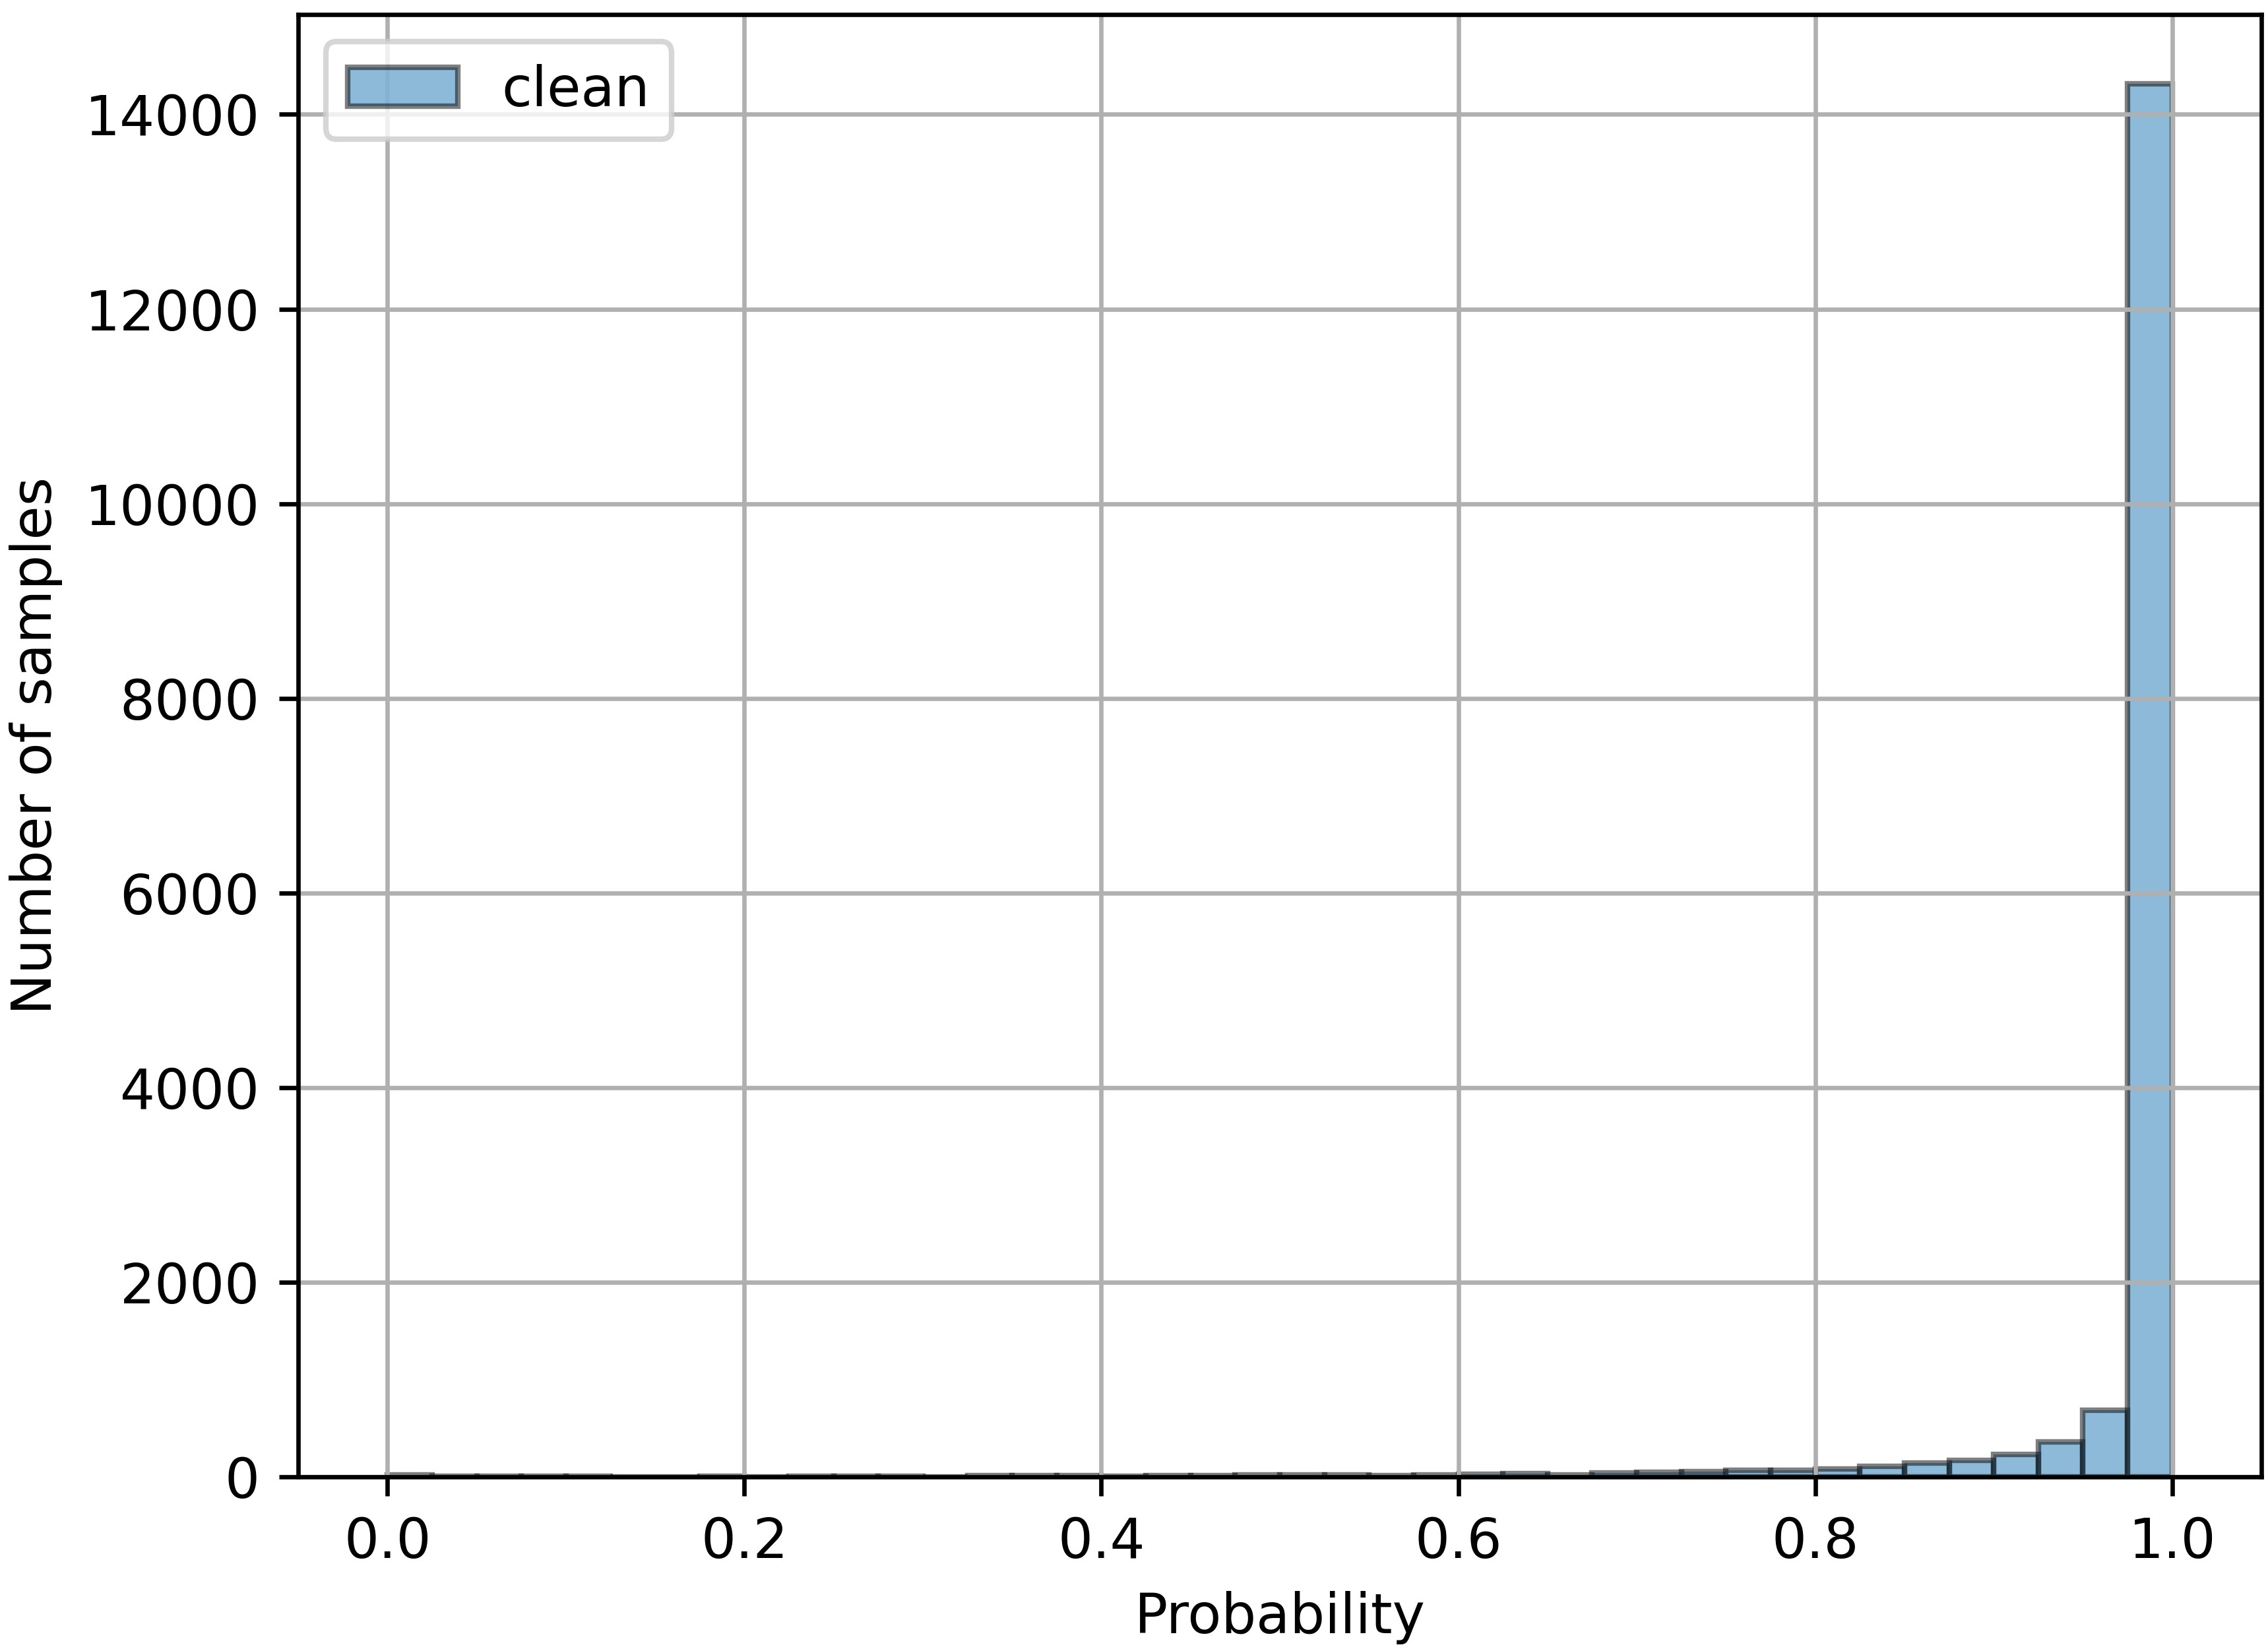}
\caption{Symmetric-Noise}
\label{NL:symm}
\end{subfigure}
% \hspace{2.25em}
\begin{subfigure}{0.317\textwidth}
\centering
\captionsetup{font=small}
\includegraphics[width=\linewidth]{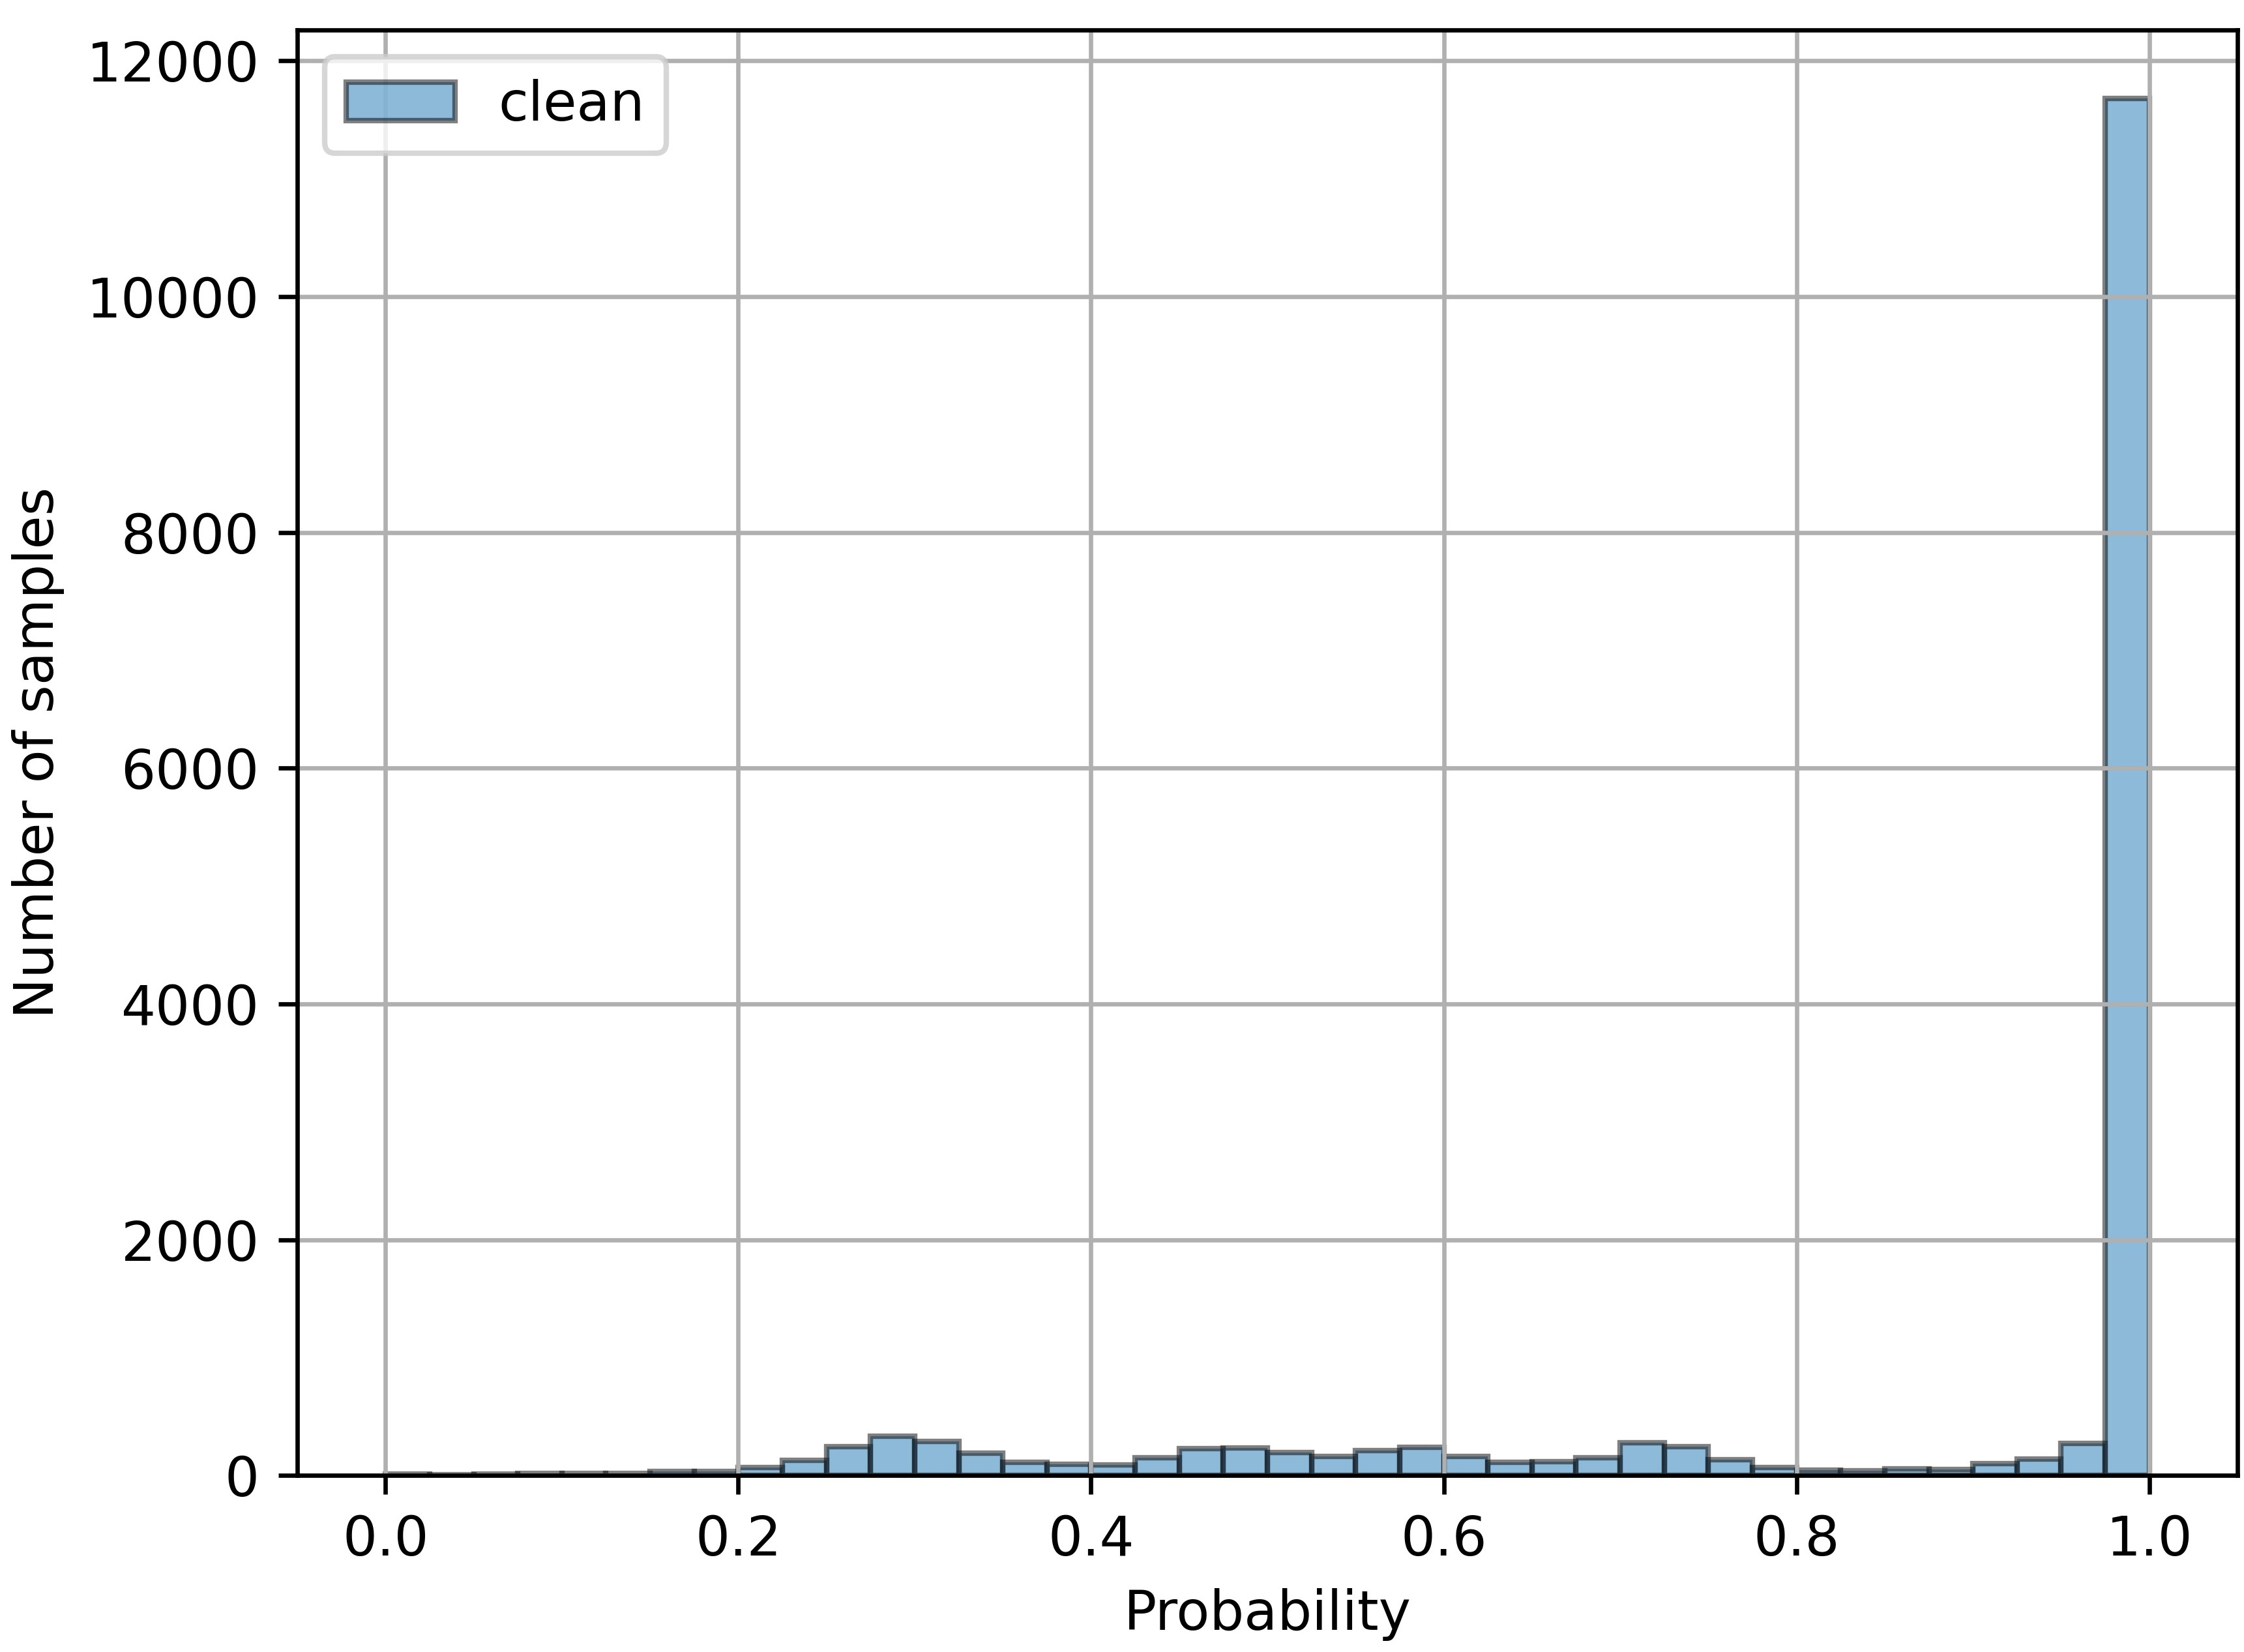}
\caption{Asymmetric-Noise}
\label{NL:asymm}
\end{subfigure}
% \hspace{2.2em}
\begin{subfigure}{0.317\textwidth}
\centering
\captionsetup{font=small}
\includegraphics[width=\linewidth]{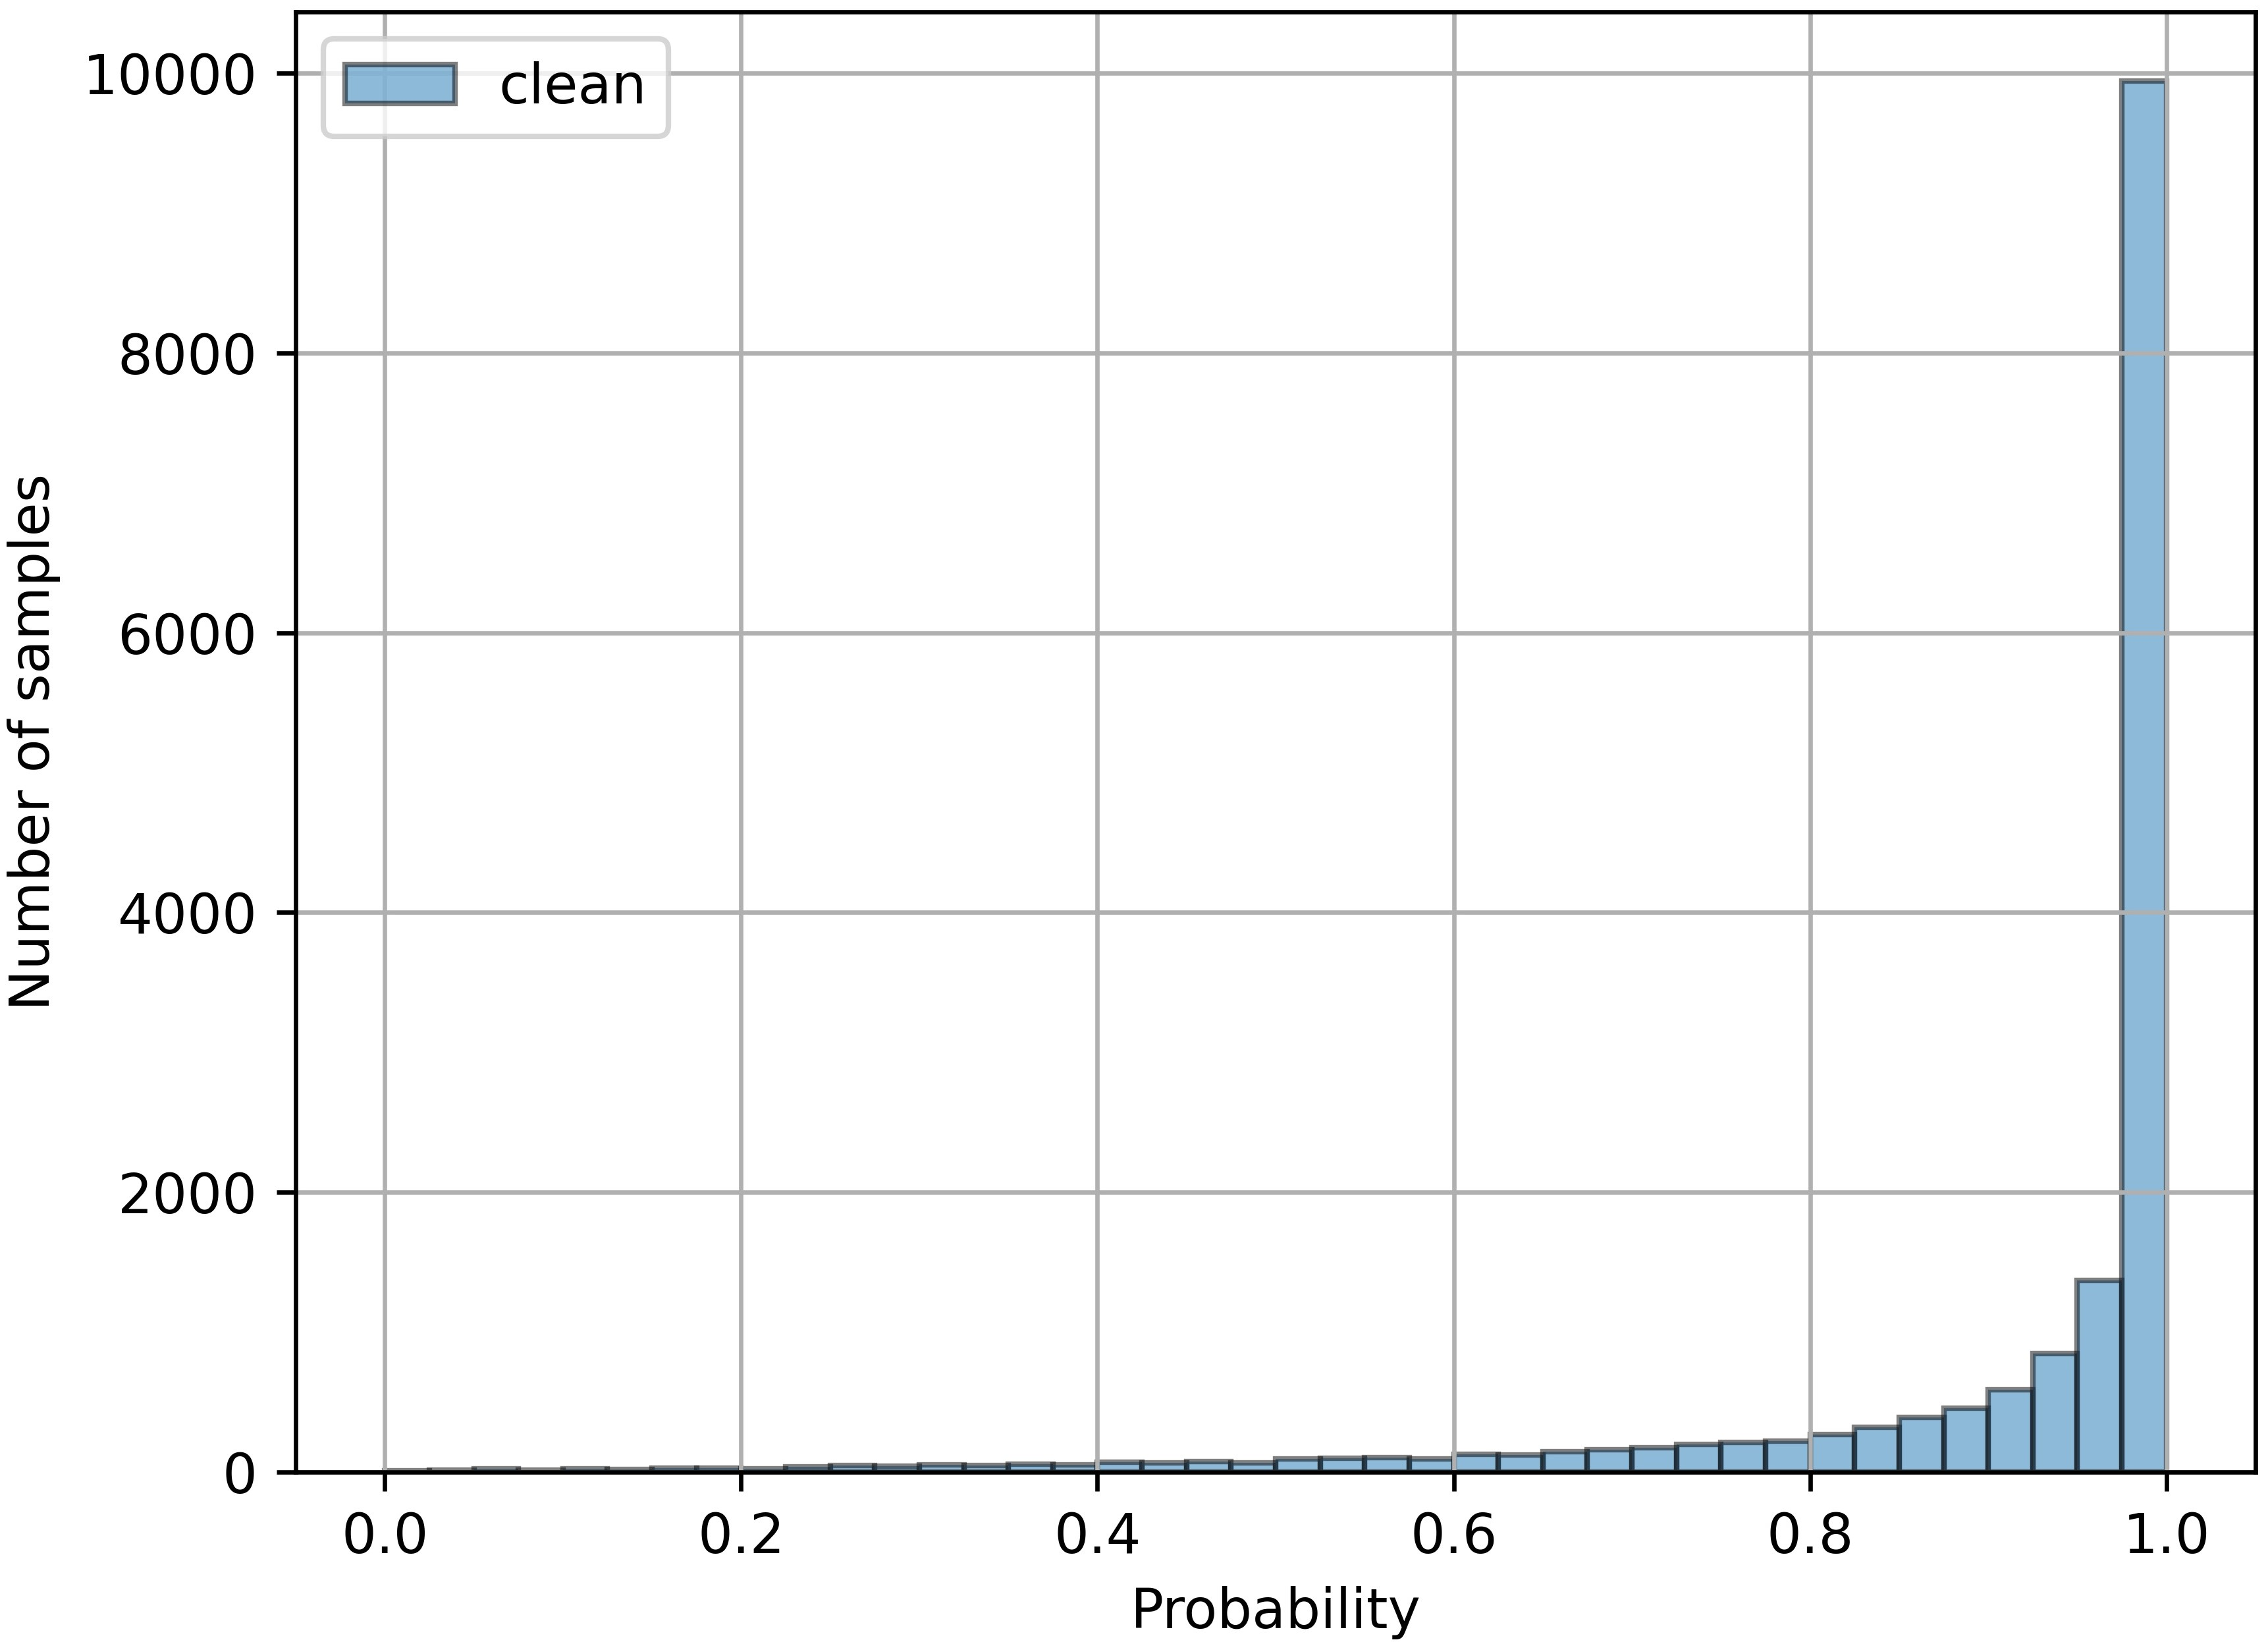}
\caption{Shift-Noise}
\label{NL:shift}
\end{subfigure}
%
% \vspace{-0.5em}
\caption{Noise filtering capability of the existing Negative Learning method \cite{kim2019nlnl} over various noise distributions. Column (a) Symmetric Noise, column (b) Asymmetric artificial noise \cite{patrini2017making}, column (c) Shift noise \cite{morerio2020generative}. First row:  the confusion matrix shows how the noise is distributed in the beginning. Second row: confidence prediction for the noisy samples after training with NL. Third row: confidence prediction for the clean samples after training with NL. The amount of initial noise is same in magnitude (\textit{i.e.,} 32.97\%) for all the cases. Note that y-scales are different in the three cases}
% \vspace{-0.5em}
\label{NL:all}
\end{figure*}
