# Supplementary material for: Continual Source-Free Unsupervised Domain Adaptation
Source: arXiv:2304.07374 source file (2023-04-14)
Supplement: Supplementary file 2 [file figure_supp_domainnet.tex]

%%%%%%%%%%%%%%%%%%%%%%%%%%%%%%%%%%%%%%%%%%%%%%%%%%%%%%%%%%%%%%%%%%%
\begin{figure*}[ht]
\captionsetup{font=small}
\centering
%%%%%%%%%%%%%%%%%%%%%%%%%%%%%%%
\begin{subfigure}{0.3\textwidth}
\centering
\captionsetup{font=small}
\includegraphics[width=\textwidth]{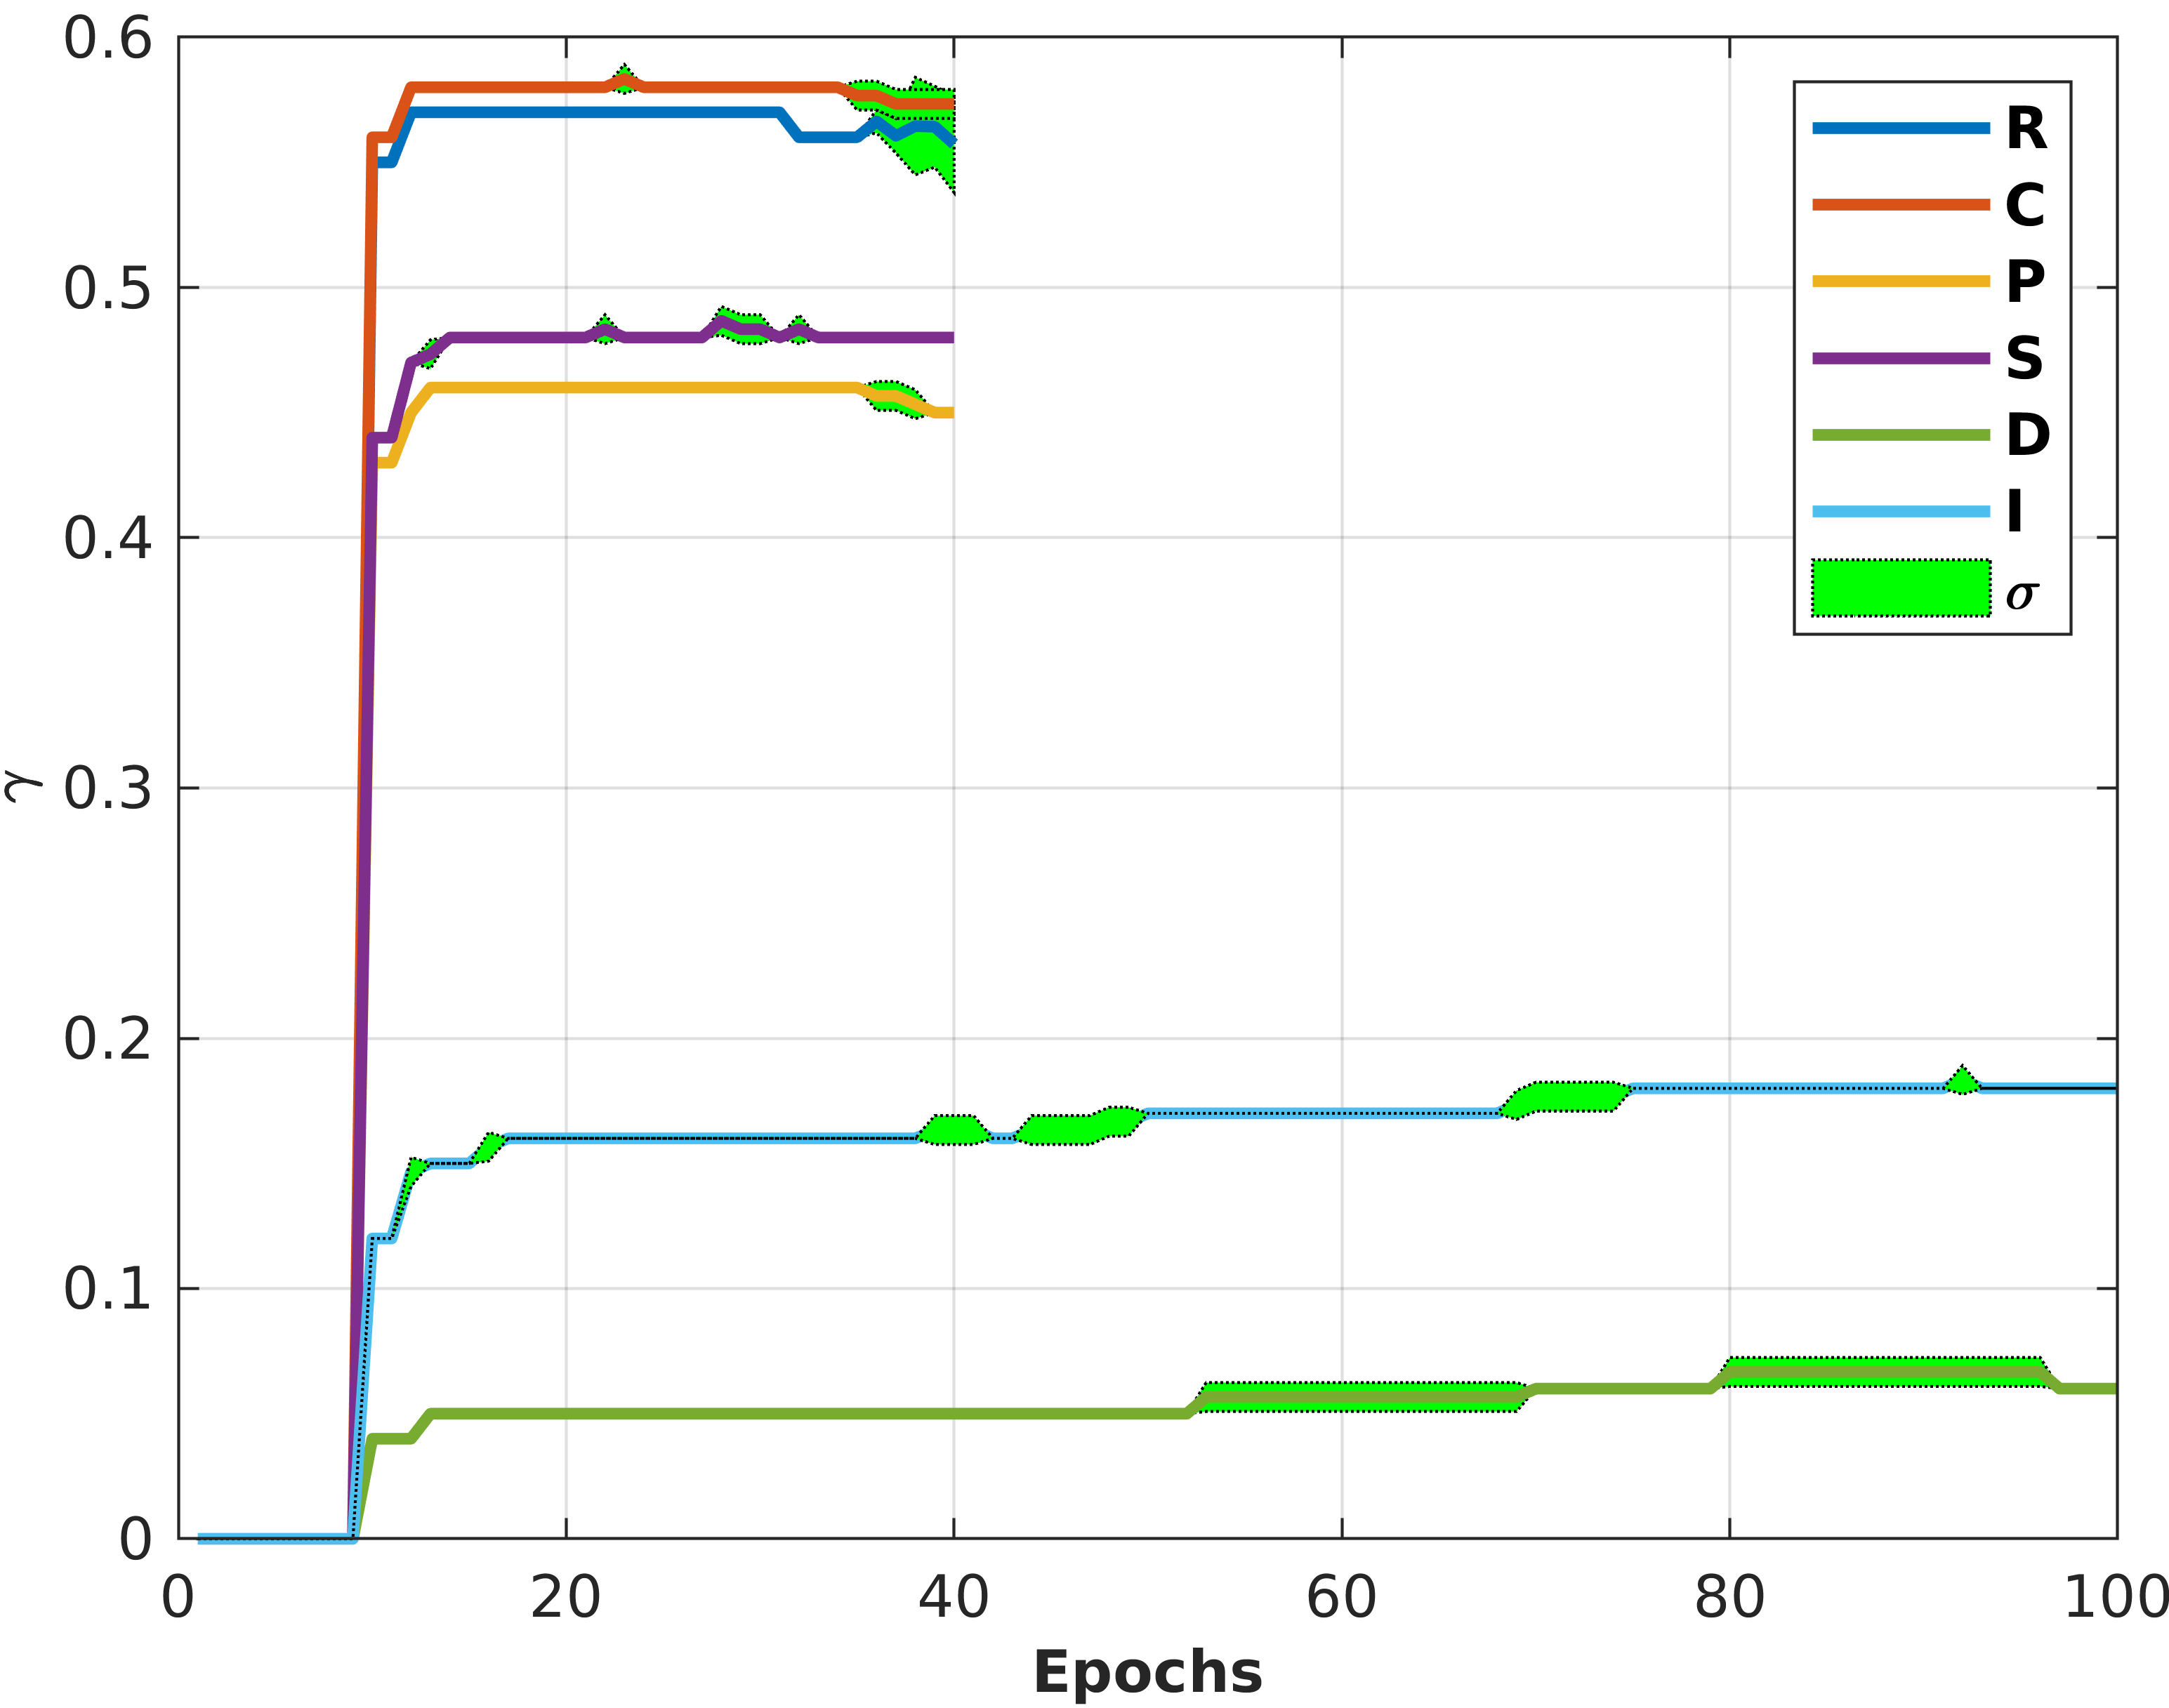}
\caption{Adaptiveness of $\gamma$ threshold.}
\label{DN:gamma}
\end{subfigure}
\begin{subfigure}{0.69\textwidth}
\centering
\captionsetup{font=small}
\includegraphics[width=\textwidth]{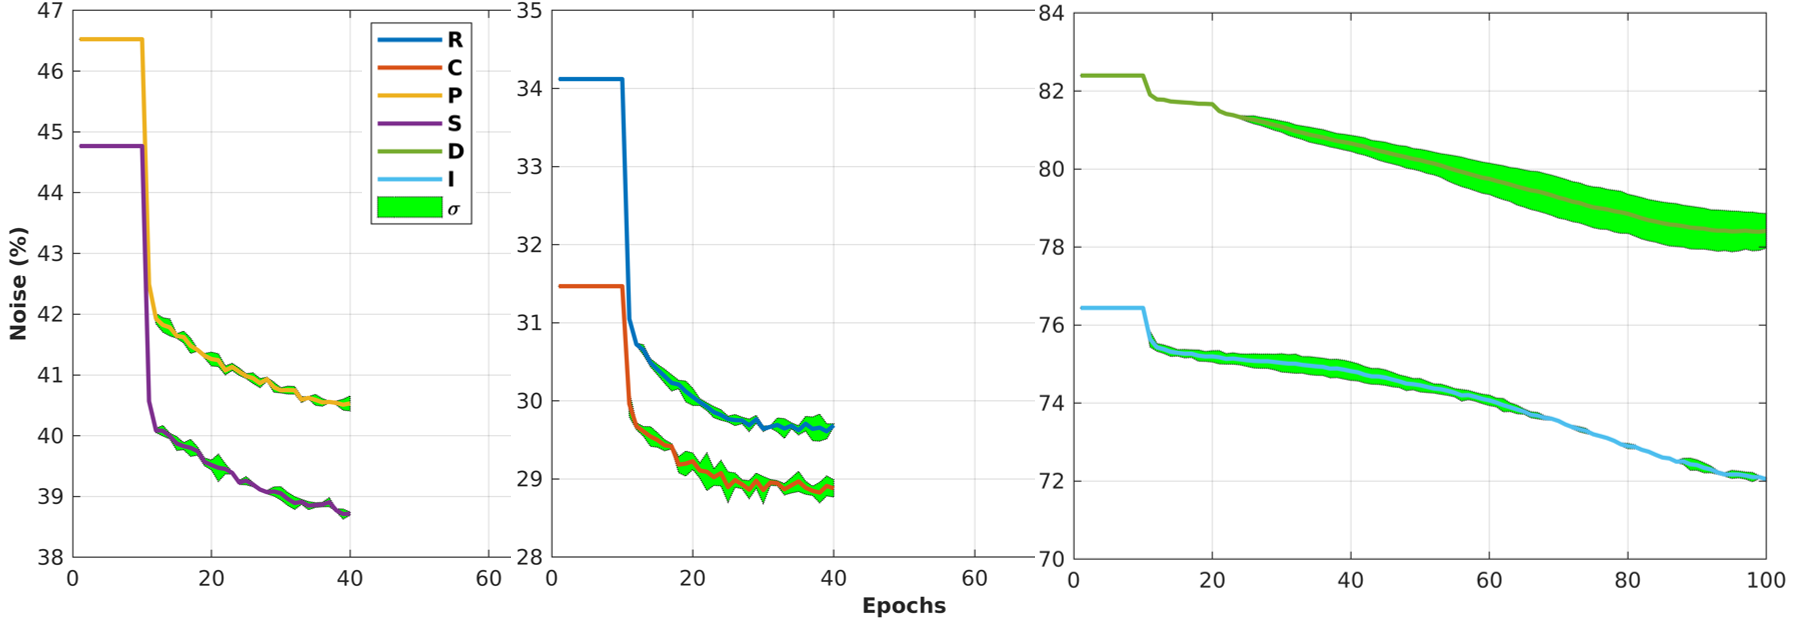}
\caption{Progressive noise reduction by pseudo-label refinement.}
\label{DN:noise}
\end{subfigure}
%
% \vspace{-0.5em}
\caption{Training evolution on DomainNet. Multi-source case: for each target, the rest of the domains are considered as source. For better representation, we concatenate noise reduction trends with different scales in (b). 
Legend: \textit{\textcolor{blue}{\textbf{C}}: Clipart, \textcolor{blue}{\textbf{I}}: Infograph, \textcolor{blue}{\textbf{P}}: Painting, \textcolor{blue}{\textbf{Q}}: Quickdraw, \textcolor{blue}{\textbf{R}}: Real, \textcolor{blue}{\textbf{S}}: Sketch, and \textcolor{blue}{\textbf{$\sigma$}}: Instantaneous standard deviation of three runs.}
}
% \vspace{-0.5em}
% \vspace{5em}
\label{DN:all}
\end{figure*}
%%%%%%%%%%%%%%%%%%%%%%%%%%%%%%%%%%%%%%%%%%%%%%%%%%%%%%%%%%%%%%%%%%%
